# Supplementary material for: Translational and rotational non-Gaussianities in homogeneous freely evolving granular gases
Source: arXiv:2303.00057 source file (2023-07-23)
Supplement: Supplementary file 1 [file SM_MS23_1_rev_v2.pdf]

# Supplementary Material to "Translational and rotational non-Gaussianities in homogeneous freely evolving granular gases"


Alberto Megías*
*Departamento de Física, Universidad de Extremadura, E-06006 Badajoz, Spain*

Andrés Santos†
*Departamento de Física, Universidad de Extremadura, E-06006 Badajoz, Spain and Instituto de Computación Científica Avanzada (ICCAEx), Universidad de Extremadura, E-06006 Badajoz, Spain*


(Dated: July 21, 2023)


In this Supplementary Material we give some helpful expressions and integrals used to compute the collisional moments, both as functions of two-body averages, and from the Sonine approximation. We also expose a comparison between the time evolution toward the HCS of the quantities $\theta$, $a_{20}$, $a_{02}$ and $a_{11}$, as predicted by the Sonine approximation, and simulation results, as well as for $\mu_{20}^{\mathrm{H}}$, $\mu_{02}^{\mathrm{H}}$, and $\langle\!\langle c_{12}\rangle\!\rangle^{\mathrm{H}}$. Finally, some details about the theoretical derivations and fitting of the high-velocity tails are developed.


## I. EVALUATION OF THE COLLISIONAL MOMENTS AS FUNCTIONS OF $d_t$ AND $d_r$

### A. Angular integrals

Some angular integrals are used in the computation of collisional moments. Here, we generalize the results for a $d$-dimensional Euclidean vector space,

$$\int_+ \mathrm{d}\widehat{\boldsymbol{\sigma}}(\mathbf{c}\cdot\widehat{\boldsymbol{\sigma}})^\ell = B_\ell c^\ell, \quad B_\ell \equiv \frac{\pi^{\frac{d_t-1}{2}}\Gamma\left(\frac{\ell+1}{2}\right)}{\Gamma\left(\frac{\ell+d_t}{2}\right)} \tag{1.1a}$$

$$\int_+ \mathrm{d}\widehat{\boldsymbol{\sigma}}(\mathbf{c}\cdot\widehat{\boldsymbol{\sigma}})^\ell \widehat{\sigma}_i = B_{\ell+1}c^{\ell-1}c_i, \tag{1.1b}$$

$$\int_+ \mathrm{d}\widehat{\boldsymbol{\sigma}}(\mathbf{c}\cdot\widehat{\boldsymbol{\sigma}})^\ell \widehat{\sigma}_i\widehat{\sigma}_j = B_{\ell+2}c^{\ell-2}c_ic_j + \frac{B_\ell - B_{\ell+2}}{d-1}c^l\delta_{ij}^\perp, \tag{1.1c}$$

$$\int_+ \mathrm{d}\widehat{\boldsymbol{\sigma}}(\mathbf{c}\cdot\widehat{\boldsymbol{\sigma}})^\ell \widehat{\sigma}_i\widehat{\sigma}_j\widehat{\sigma}_k = B_{\ell+3}c^{\ell-3}c_ic_jc_k + 3\frac{B_{\ell+1} - B_{\ell+3}}{d-1}c^{\ell-1}c_{(i}\delta_{jk)}^\perp, \tag{1.1d}$$

$$\int_+ \mathrm{d}\widehat{\boldsymbol{\sigma}}(\mathbf{c}\cdot\widehat{\boldsymbol{\sigma}})^\ell \widehat{\sigma}_i\widehat{\sigma}_j\widehat{\sigma}_k\widehat{\sigma}_m = B_{\ell+4}c^{\ell-4}c_ic_jc_kc_m + 6\frac{B_{\ell+2} - B_{\ell+4}}{d-1}c^{\ell-2}c_{(i}c_j\delta_{km)}^\perp + 3\frac{B_{\ell+4} - 2B_{\ell+2} + B_\ell}{d^2-1}c^\ell\delta_{(ij}^\perp\delta_{km)}^\perp, \tag{1.1e}$$

where $\delta_{ij}^\perp \equiv \delta_{ij} - \widehat{c}_i\widehat{c}_j$ and the notation with indices enclosed by parentheses means that one is totally symmetrizing the tensors over such indices, i.e.,

$$c_{(i}\delta_{jk)}^\perp = \frac{1}{3}\left(c_i\delta_{jk}^\perp + c_j\delta_{ik}^\perp + c_j\delta_{ij}^\perp\right), \tag{1.2a}$$

$$c_{(i}c_j\delta_{km)}^\perp = \frac{1}{6}\left(c_ic_j\delta_{km}^\perp + c_ic_k\delta_{jm}^\perp + c_ic_m\delta_{jk}^\perp + c_jc_k\delta_{im}^\perp + c_jc_m\delta_{ik}^\perp + c_kc_m\delta_{ij}^\perp\right), \tag{1.2b}$$

$$\delta_{(ij}^\perp\delta_{km)}^\perp = \frac{1}{3}\left(\delta_{ij}^\perp\delta_{km}^\perp + \delta_{ik}^\perp\delta_{jm}^\perp + \delta_{im}^\perp\delta_{jk}^\perp\right). \tag{1.2c}$$

### B. Levi-Civita summations for disks and spheres

As introduced in the main text, whereas we worked in a generalized framework, in which expressions are given in terms of the numbers of translational and rotational degrees of freedom of the problem, $d_t$ and $d_r$, respectively, we


* albertom@unex.es
† andres@unex.es

took into account only two- and three-dimensional setups. In the case of hard disks, translational velocities are vectors of a two-dimensional Euclidean space $\mathfrak{C}$, whereas the space of the angular velocities is a one-dimensional Euclidean space $\mathfrak{W}$ orthogonal to the previous one, that is, $\mathfrak{W} = \mathfrak{C}^{\perp}$, such that the total space, $\mathfrak{E}^3 = \mathfrak{C} \bigoplus \mathfrak{W}$. On the other hand, trivially for hard spheres, $\mathfrak{C} = \mathfrak{W} = \mathfrak{E}^3$. Then, we wrote all relations using general vector notation for elements in the three-dimensional Euclidean space $\mathfrak{E}^3$.

Some vector cross products appear in the computation of the collisional moments, involving both translational and angular velocity variables. Then, it is convenient to express formally those vector products in terms of the three-dimensional Levi-Civita tensor in $\mathfrak{E}^3$, $\varepsilon_{ijk}$. For example, we face terms of the kind $(\mathbf{c}\times\mathbf{w})_i = \varepsilon_{ijk}c_j w_k$, where we are using Einstein's convention of summation over repeated indices.

Let us denote by $\bar{\delta}_{ij}$ the metric of our translational Euclidean space $\mathfrak{C}$ of dimension $d_t = 2$ and 3 for disks and spheres, respectively. Therefore, if $\delta_{ij}$ is the metric of the total embedding space $\mathfrak{E}^3$, then $\bar{\delta}_{ij}\delta_{jk} = \bar{\delta}_{ik}$.

During some computations we faced expressions of the kind $\varepsilon_{ijk}\varepsilon_{ilm}$. Thus, using the identity

$$\varepsilon_{ijk}\varepsilon_{lmn} = \delta_{il}(\delta_{jm}\delta_{kn} - \delta_{jn}\delta_{km}) - \delta_{im}\delta_{jl}, \tag{1.3}$$

if the indices $i$ and $l$ are contracted by the metric in $\mathfrak{C}$, then

$$\bar{\delta}_{il}\varepsilon_{ijk}\varepsilon_{lmn} = d_t(\delta_{jm}\delta_{kn} - \delta_{jn}\delta_{km}) - (\bar{\delta}_{jm}\delta_{kn} - \delta_{jn}\bar{\delta}_{km}) - (\delta_{jm}\bar{\delta}_{kn} - \bar{\delta}_{jn}\delta_{km}), \tag{1.4}$$

where we have used that $\bar{\delta}_{ii} = d_t$.

Let us use this methodology in an example of an angular integral involving translational and rotational variables,

$$\begin{aligned}
\int_+ \mathrm{d}\widehat{\boldsymbol{\sigma}}\,(\mathbf{c}\cdot\widehat{\boldsymbol{\sigma}})^p\,[\mathbf{c}\cdot(\widehat{\boldsymbol{\sigma}}\times\mathbf{w})]^2 =& c_i c_l \left[\int_+ \mathrm{d}\widehat{\boldsymbol{\sigma}}\,(\mathbf{c}\cdot\widehat{\boldsymbol{\sigma}})^p \widehat{\sigma}_j\widehat{\sigma}_m\right]\varepsilon_{ijk}\varepsilon_{lmn}w_k w_n\\
=& c_i c_l \left[B_{p+2}c^{p-2}c_j c_m + \frac{B_p - B_{p+2}}{d_t-1}c^p\bar{\delta}^{\perp}_{jm}\right]\varepsilon_{ijk}\varepsilon_{lmn}w_k w_n\\
=& c_i c_l \left[B_{p+2}c^{p-2}c_j c_m + \frac{B_p - B_{p+2}}{d_t-1}c^p\left(\bar{\delta}_{jm} - \widehat{c}_j\widehat{c}_m\right)\right]\varepsilon_{ijk}\varepsilon_{lmn}w_k w_n\\
=& B_{p+2}c^{p-2}[\mathbf{c}\cdot(\mathbf{c}\times\mathbf{w})]^2 + \frac{B_p - B_{p+2}}{d_t-1}\Big\{c^p\left[d_t(\delta_{il}\delta_{kn} - \delta_{in}\delta_{kl})\right.\\
&\left. -(\bar{\delta}_{il}\delta_{kn} - \delta_{in}\bar{\delta}_{kl}) - (\delta_{il}\bar{\delta}_{kn} - \bar{\delta}_{in}\delta_{kl})\right]c_i c_l w_k w_n - c^{p-2}[\mathbf{c}\cdot(\mathbf{c}\times\mathbf{w})]^2\Big\}\\
=& \frac{B_p - B_{p+2}}{d_t-1}c^p\left[d_t(\delta_{il}\delta_{kn} - \delta_{in}\delta_{kl}) - (\bar{\delta}_{il}\delta_{kn} - \delta_{in}\bar{\delta}_{kl}) - (\delta_{il}\bar{\delta}_{kn} - \bar{\delta}_{in}\delta_{kl})\right]c_i c_l w_k w_n\\
=& \frac{B_p - B_{p+2}}{d_t-1}\left[c^{p+2}w^2 - (4-d_t)c^p(\mathbf{c}\cdot\mathbf{w})^2\right].
\end{aligned} \tag{1.5}$$

For disks ($d_t = 2$, $d_r = 1$), we have $\mathbf{c}\perp\mathbf{w}$, so that the second term vanishes. Then, one can simply replace $(4-d_t)c^p(\mathbf{c}\cdot\mathbf{w})^2$ by $\frac{d_r-1}{2}c^p(\mathbf{c}\cdot\mathbf{w})^2$, which holds both for hard disks and hard spheres. Following the same reasoning, one gets, for instance,

$$\begin{aligned}
\int_+ \mathrm{d}\widehat{\boldsymbol{\sigma}}\,(\mathbf{c}_{12}\cdot\widehat{\boldsymbol{\sigma}})^p\,[\mathbf{C}_{12}\cdot(\widehat{\boldsymbol{\sigma}}\times\mathbf{W}_{12})]^2 =& \left(B_{p+2} - \frac{B_p - B_{p+2}}{d_t-1}\right)c_{12}^p[\mathbf{C}_{12}\cdot(\mathbf{c}_{12}\times\mathbf{W}_{12})]^2\\
&+ \frac{B_p - B_{p+2}}{d_t-1}\left[c_{12}^p C_{12}^2 W_{12}^2 - \frac{d_r-1}{2}c_{12}^p(\mathbf{C}_{12}\cdot\mathbf{W}_{12})^2\right],
\end{aligned} \tag{1.6}$$

where we have called $C_{12} \equiv \frac{1}{2}(\mathbf{c}_1 + \mathbf{c}_2)$.

### C. Computations of collisional moments

#### 1. Collisional impulse

In Sec. II B of the main paper we expressed the postcollisional velocities in terms of the (reduced) impulse $\boldsymbol{\Delta}_{12}$. It is then possible to derive the following results:

$$\boldsymbol{\Delta}_{12}^2 =\overline{\alpha}^2(\mathbf{c}_{12}\cdot\widehat{\boldsymbol{\sigma}})^2+\overline{\beta}^2[c_{12}^2-(\mathbf{c}_{12}\cdot\widehat{\boldsymbol{\sigma}})^2+4\frac{\theta}{\kappa}(\widehat{\boldsymbol{\sigma}}\times\mathbf{W}_{12})^2-4\sqrt{\frac{\theta}{\kappa}}\mathbf{c}_{12}\cdot(\widehat{\boldsymbol{\sigma}}\times\mathbf{W}_{12})], \tag{1.7a}$$

$$\widehat{\boldsymbol{\sigma}}\cdot\boldsymbol{\Delta}_{12} =\overline{\alpha}(\mathbf{c}_{12}\cdot\widehat{\boldsymbol{\sigma}}), \tag{1.7b}$$

$$\begin{aligned}\boldsymbol{\Delta}_{12}^4 =&\overline{\alpha}^4(\mathbf{c}_{12}\cdot\widehat{\boldsymbol{\sigma}})^4+\overline{\beta}^4\left\{c_{12}^4+(\mathbf{c}_{12}\cdot\widehat{\boldsymbol{\sigma}})^4-2c_{12}^2(\mathbf{c}_{12}\cdot\widehat{\boldsymbol{\sigma}})^2+16\frac{\theta^2}{\kappa^2}\left[W_{12}^4+(\widehat{\boldsymbol{\sigma}}\cdot\mathbf{W}_{12})^4-2W_{12}^2(\widehat{\boldsymbol{\sigma}}\cdot\mathbf{W}_{12})^2\right]\right.\\&+16\frac{\theta}{\kappa}\left[\mathbf{c}_{12}\cdot(\widehat{\boldsymbol{\sigma}}\times\mathbf{W}_{12})\right]^2-8\sqrt{\frac{\theta}{\kappa}}\left[\mathbf{c}_{12}\cdot(\widehat{\boldsymbol{\sigma}}\times\mathbf{W}_{12})\right]\left[c_{12}^2-(\mathbf{c}_{12}\cdot\widehat{\boldsymbol{\sigma}})^2+\frac{4\theta}{\kappa}(\widehat{\boldsymbol{\sigma}}\times\mathbf{W}_{12})^2\right]\\&\left.+8\frac{\theta}{\kappa}[W_{12}^2-(\mathbf{W}_{12}\cdot\widehat{\boldsymbol{\sigma}})^2][c_{12}^2-(\mathbf{c}_{12}\cdot\widehat{\boldsymbol{\sigma}})^2]\right\}+2\overline{\alpha}^2\overline{\beta}^2\left\{c_{12}^2(\mathbf{c}_{12}\cdot\widehat{\boldsymbol{\sigma}})^2-(\mathbf{c}_{12}\cdot\widehat{\boldsymbol{\sigma}})^4\right.\\&\left.+4\frac{\theta}{\kappa}[W_{12}^2-(\widehat{\boldsymbol{\sigma}}\cdot\mathbf{W}_{12})^2](\mathbf{c}_{12}\cdot\widehat{\boldsymbol{\sigma}})^2\right\},\end{aligned}$$

$$\begin{aligned}\boldsymbol{\Delta}_{12}^2(\widehat{\boldsymbol{\sigma}}\cdot\boldsymbol{\Delta}_{12})^2 =&\overline{\alpha}^4(\mathbf{c}_{12}\cdot\widehat{\boldsymbol{\sigma}})^4+\overline{\beta}^2\overline{\alpha}^2\left\{c_{12}^2(\mathbf{c}_{12}\cdot\widehat{\boldsymbol{\sigma}})^2-(\mathbf{c}_{12}\cdot\widehat{\boldsymbol{\sigma}})^4+4\frac{\theta}{\kappa}\left[W_{12}^2-(\widehat{\boldsymbol{\sigma}}\cdot\mathbf{W}_{12})^2\right](\mathbf{c}_{12}\cdot\widehat{\boldsymbol{\sigma}})^2\right.\\&\left.-4\sqrt{\frac{\theta}{\kappa}}(\mathbf{c}_{12}\cdot\widehat{\boldsymbol{\sigma}})\left[\mathbf{c}_{12}\cdot(\widehat{\boldsymbol{\sigma}}\times\mathbf{W}_{12})\right]\right\},\end{aligned} \tag{1.7c}$$

$$\widehat{\boldsymbol{\sigma}}\times\boldsymbol{\Delta}_{12} =\overline{\beta}\left\{(\widehat{\boldsymbol{\sigma}}\times\mathbf{c}_{12})+2\sqrt{\frac{\theta}{\kappa}}[\mathbf{W}_{12}-(\widehat{\boldsymbol{\sigma}}\cdot\mathbf{W}_{12})\widehat{\boldsymbol{\sigma}}]\right\}, \tag{1.7d}$$

$$\mathbf{c}_{12}\cdot\boldsymbol{\Delta}_{12} =\overline{\alpha}(\mathbf{c}_{12}\cdot\widehat{\boldsymbol{\sigma}})^2+\overline{\beta}\left[c_{12}^2-(\mathbf{c}_{12}\cdot\widehat{\boldsymbol{\sigma}})^2-2\sqrt{\frac{\theta}{\kappa}}\mathbf{c}_{12}\cdot(\widehat{\boldsymbol{\sigma}}\times\mathbf{W}_{12})\right], \tag{1.7e}$$

$$\mathbf{C}_{12}\cdot\boldsymbol{\Delta}_{12} =\overline{\alpha}(\mathbf{c}_{12}\cdot\widehat{\boldsymbol{\sigma}})(\mathbf{C}_{12}\cdot\widehat{\boldsymbol{\sigma}})+\overline{\beta}\left[\mathbf{c}_{12}\cdot\mathbf{C}_{12}-(\mathbf{c}_{12}\cdot\widehat{\boldsymbol{\sigma}})(\mathbf{C}_{12}\cdot\widehat{\boldsymbol{\sigma}})-2\sqrt{\frac{\theta}{\kappa}}\mathbf{C}_{12}\cdot(\widehat{\boldsymbol{\sigma}}\times\mathbf{W}_{12})\right], \tag{1.7f}$$

where use has been made the following vector relations,

$$\widehat{\boldsymbol{\sigma}}\times(\widehat{\boldsymbol{\sigma}}\times\mathbf{A})=(\widehat{\boldsymbol{\sigma}}\times\mathbf{A})\widehat{\boldsymbol{\sigma}}-\mathbf{A},\qquad(\widehat{\boldsymbol{\sigma}}\times\mathbf{A})\cdot(\widehat{\boldsymbol{\sigma}}\times\mathbf{B})=\mathbf{A}\cdot\mathbf{B}-(\widehat{\boldsymbol{\sigma}}\cdot\mathbf{A})(\widehat{\boldsymbol{\sigma}}\cdot\mathbf{B}). \tag{1.8}$$

#### 2. Collisional changes

As seen in the main text, the (reduced) collisional moments can be written as

$$\mu_{pq}^{(r)}=-\frac{1}{2}\int\mathrm{d}\widetilde{\boldsymbol{\Gamma}}_1\int\mathrm{d}\widetilde{\boldsymbol{\Gamma}}_2\int_+\mathrm{d}\widehat{\boldsymbol{\sigma}}\,(\mathbf{c}_{12}\cdot\widehat{\boldsymbol{\sigma}})\phi(\widetilde{\boldsymbol{\Gamma}}_1)\phi(\widetilde{\boldsymbol{\Gamma}}_2)(\mathcal{B}_{12,\widehat{\boldsymbol{\sigma}}}-1)\left[\psi_{pq}^{(r)}(\widetilde{\boldsymbol{\Gamma}}_1)+\psi_{pq}^{(r)}(\widetilde{\boldsymbol{\Gamma}}_2)\right],\quad\psi_{pq}^{(r)}(\widetilde{\boldsymbol{\Gamma}})\equiv c^pw^q(\mathbf{c}\cdot\mathbf{w})^r. \tag{1.9}$$

Using Eqs. (1.7a), we have obtained the collisional changes associated with the second- and fourth-order collisional moments. They are displayed in Table I.

#### 3. Collisional moments in terms of two-body averages

Once the collisional changes displayed in Table I are inserted into Eq. (1.9) and the angular integrals are performed (see Sec. I A), the collisional moments can be expressed in terms of two-body averages. The results are listed in Table II, where, as in the main text, we have simplified the notation as $\mu_{pq}^{(0)}\to\mu_{pq}$. We do not include $\mu_{00}^{(2)}$ because it is meaningful only for hard spheres and is already known.[1]

TABLE I. Collisional changes of the quantities $\psi_{pq}^{(r)}(\widetilde{\mathbf{\Gamma}})$ with $p+q+2r=2$ and 4.

| $(p,q,r)$ | $\psi_{pq}^{(r)}(\widetilde{\mathbf{\Gamma}})$ | $(\mathcal{B}_{12,\widehat{\boldsymbol{\sigma}}}-1)\left[\psi_{pq}^{(r)}(\widetilde{\mathbf{\Gamma}}_1)+\psi_{pq}^{(r)}(\widetilde{\mathbf{\Gamma}}_2)\right]$ |
|---|---|---|
| $(2,0,0)$ | $c^2$ | $2\left[\boldsymbol{\Delta}_{12}^2-(\mathbf{c}_{12}\cdot\boldsymbol{\Delta}_{12})\right]$ |
| $(0,2,0)$ | $w^2$ | $\frac{2}{\kappa\theta}\left[\boldsymbol{\Delta}_{12}^2-(\widehat{\boldsymbol{\sigma}}\cdot\boldsymbol{\Delta}_{12})^2\right]-\frac{4}{\sqrt{\kappa\theta}}\mathbf{W}_{12}\cdot(\widehat{\boldsymbol{\sigma}}\times\boldsymbol{\Delta}_{12})$ |
| $(4,0,0)$ | $c^4$ | $2\boldsymbol{\Delta}_{12}^4+2\left[(\mathbf{c}_{12}\cdot\boldsymbol{\Delta}_{12})^2+4(\mathbf{C}_{12}\cdot\boldsymbol{\Delta}_{12})^2\right]+\boldsymbol{\Delta}_{12}^2(c_{12}^2+4C_{12}^2)-4\boldsymbol{\Delta}_{12}^2(\mathbf{c}_{12}\cdot\boldsymbol{\Delta}_{12})-8(\mathbf{C}_{12}\cdot\boldsymbol{\Delta}_{12})(\mathbf{c}_{12}\cdot\mathbf{C}_{12})$ $-(c_{12}^2+4C_{12}^2)(\mathbf{c}_{12}\cdot\boldsymbol{\Delta}_{12})$ |
| $(0,4,0)$ | $w^4$ | $\frac{2}{\kappa^2\theta^2}\left[\boldsymbol{\Delta}_{12}^4+(\widehat{\boldsymbol{\sigma}}\cdot\boldsymbol{\Delta}_{12})^4-2\boldsymbol{\Delta}_{12}^2(\widehat{\boldsymbol{\sigma}}\cdot\boldsymbol{\Delta}_{12})^2\right]+\frac{2}{\kappa\theta}\Bigg\{4[\mathbf{W}_{12}\cdot(\widehat{\boldsymbol{\sigma}}\times\boldsymbol{\Delta}_{12})]^2+[\mathbf{w}_{12}\cdot(\widehat{\boldsymbol{\sigma}}\times\boldsymbol{\Delta}_{12})]^2+\left(2W_{12}^2+\frac{w_{12}^2}{2}\right)$ $\times\left[\boldsymbol{\Delta}_{12}^2-(\widehat{\boldsymbol{\sigma}}\cdot\boldsymbol{\Delta}_{12})^2\right]\Bigg\}-\frac{4}{\sqrt{\kappa\theta}}\left[\left(2W_{12}^2+\frac{w_{12}^2}{2}\right)\mathbf{W}_{12}\cdot(\widehat{\boldsymbol{\sigma}}\times\boldsymbol{\Delta}_{12})+(\mathbf{W}_{12}\cdot\mathbf{w}_{12})\,\mathbf{w}_{12}\cdot(\widehat{\boldsymbol{\sigma}}\times\boldsymbol{\Delta}_{12})\right]$ $-\frac{8}{\kappa\theta\sqrt{\kappa\theta}}\left[\boldsymbol{\Delta}_{12}^2-(\widehat{\boldsymbol{\sigma}}\cdot\boldsymbol{\Delta}_{12})^2\right]\mathbf{W}_{12}\cdot(\widehat{\boldsymbol{\sigma}}\times\boldsymbol{\Delta}_{12})$ |
| $(2,2,0)$ | $c^2w^2$ | $\frac{1}{\kappa\theta}\left[\boldsymbol{\Delta}_{12}^2-(\widehat{\boldsymbol{\sigma}}\cdot\boldsymbol{\Delta}_{12})^2\right]\left\{\frac{1}{2}(4C_{12}^2+c_{12}^2)+2[\boldsymbol{\Delta}_{12}^2-(\mathbf{c}_{12}\cdot\boldsymbol{\Delta}_{12})]\right\}+\frac{2}{\sqrt{\kappa\theta}}\Bigg\{\mathbf{C}_{12}\cdot(2\boldsymbol{\Delta}_{12}-\mathbf{c}_{12})\left[\mathbf{w}_{12}\cdot(\widehat{\boldsymbol{\sigma}}\times\boldsymbol{\Delta}_{12})\right]$ $-\frac{1}{2}\left[4C_{12}^2+c_{12}^2+4(\boldsymbol{\Delta}_{12}^2-\mathbf{c}_{12}\cdot\boldsymbol{\Delta}_{12})\right]\left[\mathbf{W}_{12}\cdot(\widehat{\boldsymbol{\sigma}}\times\boldsymbol{\Delta}_{12})\right]\Bigg\}+\frac{1}{2}\left(4W_{12}^2+w_{12}^2\right)\left[\boldsymbol{\Delta}_{12}^2-(\mathbf{c}_{12}\cdot\boldsymbol{\Delta}_{12})\right]$ $-4\left(\mathbf{W}_{12}\cdot\mathbf{w}_{12}\right)\left(\mathbf{C}_{12}\cdot\boldsymbol{\Delta}_{12}\right)$ |
| $(0,0,2)$ | $(\mathbf{c}\cdot\mathbf{w})^2$ | $2(\mathbf{W}_{12}\cdot\boldsymbol{\Delta}_{12})^2+\frac{1}{2}(\mathbf{w}_{12}\cdot\boldsymbol{\Delta}_{12})^2+\frac{2}{\kappa\theta}\left\{[\mathbf{C}_{12}\cdot(\widehat{\boldsymbol{\sigma}}\times\boldsymbol{\Delta}_{12})]^2+\frac{1}{4}[\mathbf{c}_{12}\cdot(\widehat{\boldsymbol{\sigma}}\times\boldsymbol{\Delta}_{12})]^2\right\}-2\left(\mathbf{C}_{12}\cdot\mathbf{w}_{12}+\mathbf{W}_{12}\cdot\mathbf{c}_{12}\right)$ $\times\left(\mathbf{W}_{12}\cdot\boldsymbol{\Delta}_{12}\right)-2\left(\mathbf{C}_{12}\cdot\mathbf{W}_{12}+\frac{1}{4}\mathbf{c}_{12}\cdot\mathbf{w}_{12}\right)(\mathbf{w}_{12}\cdot\boldsymbol{\Delta}_{12})+\frac{2}{\sqrt{\kappa\theta}}\Big\{(\mathbf{W}_{12}\cdot\boldsymbol{\Delta}_{12})\left[\mathbf{c}_{12}\cdot(\widehat{\boldsymbol{\sigma}}\times\boldsymbol{\Delta}_{12})\right]+(\mathbf{w}_{12}\cdot\boldsymbol{\Delta}_{12})$ $\times\left[\mathbf{C}_{12}\cdot(\widehat{\boldsymbol{\sigma}}\times\boldsymbol{\Delta}_{12})\right]-\left[2(\mathbf{C}_{12}\cdot\mathbf{W}_{12})+\frac{1}{2}(\mathbf{c}_{12}\cdot\mathbf{w}_{12})\right]\mathbf{C}_{12}\cdot(\widehat{\boldsymbol{\sigma}}\times\boldsymbol{\Delta}_{12})-\frac{1}{2}\left[(\mathbf{C}_{12}\cdot\mathbf{w}_{12})+(\mathbf{W}_{12}\cdot\mathbf{c}_{12})\right]\mathbf{c}_{12}\cdot(\widehat{\boldsymbol{\sigma}}\times\boldsymbol{\Delta}_{12})\Big\}$ |

Upon derivation of the results of Table II, we have needed to take into account the following relations:

$$\begin{aligned}\frac{\langle\!\langle\boldsymbol{\Delta}_{12}^4\rangle\!\rangle}{2B_5}=&\frac{1}{2}\left(\overline{\alpha}^4+\overline{\beta}^4\frac{d_t^2-1}{8}+\overline{\alpha}^2\overline{\beta}^2\frac{d_t-1}{2}\right)\langle\!\langle c_{12}^5\rangle\!\rangle+\frac{\theta^2}{\kappa^2}\overline{\beta}^4\left[15\langle\!\langle c_{12}W_{12}^4\rangle\!\rangle-2d_t\langle\!\langle c_{12}^{-1}W_{12}^2(\mathbf{c}_{12}\cdot\mathbf{W}_{12})^2\rangle\!\rangle\right.\\&\left.-\langle\!\langle c_{12}^{-3}(\mathbf{c}_{12}\cdot\mathbf{W}_{12})^4\rangle\!\rangle\right]+\frac{\theta\overline{\beta}^2}{2\kappa}\left[\overline{\beta}^2(d_t+1)-\overline{\alpha}^2\right]\left[5\langle\!\langle c_{12}^3W_{12}^2\rangle\!\rangle-3\langle\!\langle c_{12}(\mathbf{c}_{12}\cdot\mathbf{W}_{12})^2\rangle\!\rangle\right],\end{aligned}\tag{1.10a}$$

$$\begin{aligned}\frac{\langle\!\langle\boldsymbol{\Delta}_{12}^2(4C_{12}^2+c_{12}^2)\rangle\!\rangle}{2B_5}=&\frac{d_t+3}{8}\Bigg\{\left(\overline{\alpha}^2+\overline{\beta}^2\frac{d_t-1}{2}\right)\langle\!\langle c_{12}^3(c_{12}^2+4C_{12}^2)\rangle\!\rangle+2\overline{\beta}^2\frac{\theta}{\kappa}\left[3\langle\!\langle c_{12}W_{12}^2(c_{12}^2+4C_{12}^2)\rangle\!\rangle\right.\\&\left.-\langle\!\langle c_{12}^{-1}(\mathbf{c}_{12}\cdot\mathbf{W}_{12})^2(c_{12}^2+4C_{12}^2)\rangle\!\rangle\right]\Bigg\},\end{aligned}\tag{1.10b}$$

$$\frac{\langle\!\langle(\mathbf{c}_{12}\cdot\boldsymbol{\Delta}_{12})^2\rangle\!\rangle}{2B_5}=\frac{1}{2}\left(\overline{\alpha}^2+\overline{\beta}^2\frac{d_t^2-1}{8}+\overline{\alpha}\overline{\beta}\frac{d_t-1}{2}\right)\langle\!\langle c_{12}^5\rangle\!\rangle+\overline{\beta}^2\frac{\theta}{\kappa}\frac{d_t+3}{4}\left[\langle\!\langle c_{12}^3W_{12}^2\rangle\!\rangle-\langle\!\langle c_{12}(\mathbf{c}_{12}\cdot\mathbf{W}_{12})^2\rangle\!\rangle\right],\tag{1.10c}$$

$$\begin{aligned}\frac{\langle\!\langle(\mathbf{C}_{12}\cdot\boldsymbol{\Delta}_{12})(4C_{12}^2+c_{12}^2)\rangle\!\rangle}{2B_5}=&\frac{d_t+3}{8}\left(\overline{\alpha}+\overline{\beta}\frac{d_t-1}{2}\right)\langle\!\langle c_{12}(\mathbf{c}_{12}\cdot\mathbf{C}_{12})(4C_{12}^2+c_{12}^2)\rangle\!\rangle\\&-\overline{\beta}\sqrt{\frac{\theta}{\kappa}}\frac{B_2}{B_5}\langle\!\langle(4C_{12}^2+c_{12}^2)\mathbf{C}_{12}\cdot(\mathbf{c}_{12}\times\mathbf{W}_{12})\rangle\!\rangle,\end{aligned}\tag{1.10d}$$

$$\begin{aligned}\frac{\langle\!\langle\boldsymbol{\Delta}_{12}^2(\mathbf{c}_{12}\cdot\boldsymbol{\Delta}_{12})\rangle\!\rangle}{2B_5}=&\frac{1}{2}\left[\overline{\alpha}^3+\frac{d_t-1}{4}\left(\overline{\alpha}\overline{\beta}^2+\overline{\alpha}^2\overline{\beta}\right)+\frac{d_t^2-1}{8}\overline{\beta}^3\right]\langle\!\langle c_{12}^5\rangle\!\rangle\\&+\frac{1}{2}\frac{\theta}{\kappa}\overline{\beta}^2\left\{\left[5\overline{\alpha}+\left(\frac{3d_t-1}{2}+(d_t+3)\right)\overline{\beta}\right]\langle\!\langle c_{12}^3W_{12}^2\rangle\!\rangle-\left[3\overline{\alpha}+\left(\frac{d_t-3}{2}+(d_t+3)\right)\overline{\beta}\right]\right.\\&\left.\times\langle\!\langle c_{12}(\mathbf{c}_{12}\cdot\mathbf{W}_{12})^2\rangle\!\rangle\right\},\end{aligned}\tag{1.10e}$$

TABLE II. Collisional moments $\mu_{pq}$ with $p+q=2$ and 4 in terms of two-body averages.

| $(p,q)$ | $-\mu_{pq}/B_5$ |
|---|---|
| $(2,0)$ | $\frac{d_t+3}{4}\Big\{\Big[\overline{\alpha}(\overline{\alpha}-1)+\frac{d_t-1}{2}\overline{\beta}(\overline{\beta}-1)\Big]\langle\langle c_{12}^3\rangle\rangle+2\overline{\beta}^2\frac{\theta}{\kappa}\Big[3\langle\langle c_{12}W_{12}^2\rangle\rangle-\langle\langle c_{12}^{-1}(\mathbf{c}_{12}\cdot\mathbf{W}_{12})^2\rangle\rangle\Big]\Big\}$ |
| $(0,2)$ | $\frac{d_t+3}{4}\frac{\overline{\beta}}{\kappa}\Big\{-2\Big(1-\frac{\overline{\beta}}{\kappa}\Big)\Big[3\langle\langle c_{12}W_{12}^2\rangle\rangle-\langle\langle c_{12}^{-1}(\mathbf{c}_{12}\cdot\mathbf{W}_{12})^2\rangle\rangle\Big]+\frac{\overline{\beta}}{\theta}\frac{d_t-1}{2}\langle\langle c_{12}^3\rangle\rangle\Big\}$ |
| $(4,0)$ | $\Big\{\overline{\alpha}^3(\overline{\alpha}-2)+\frac{d_t^2-1}{8}\overline{\beta}^3(\overline{\beta}-2)+\frac{d_t-1}{2}\overline{\alpha}\overline{\beta}(\overline{\alpha}\overline{\beta}-\overline{\alpha}-\overline{\beta}+1)+\frac{d_t+3}{8}\Big[\overline{\alpha}(2\overline{\alpha}-1)+\frac{d_t-1}{2}\overline{\beta}(2\overline{\beta}-1)\Big]+\overline{\alpha}^2+\frac{d_t^2-1}{8}\overline{\beta}^2\Big\}\langle\langle c_{12}^5\rangle\rangle$ |
| | $+\Big\{(\overline{\alpha}-\overline{\beta})^2+\frac{d_t+3}{2}\Big[\overline{\alpha}(\overline{\alpha}-1)+\frac{d_t-1}{2}\overline{\beta}(\overline{\beta}-1)\Big]\Big\}\langle\langle c_{12}^3C_{12}^2\rangle\rangle+\Big\{3\overline{\alpha}(\overline{\alpha}-1)+\frac{d_t-1}{2}\overline{\beta}\Big[(d_t+3)\overline{\beta}-3\Big]+d_t\Big[2\overline{\beta}(\overline{\alpha}-\overline{\beta})-\overline{\alpha}-\overline{\beta}\frac{d_t-1}{2}\Big]\Big\}\langle\langle c_{12}(\mathbf{c}_{12}\cdot\mathbf{C}_{12})^2\rangle\rangle+2\frac{\theta}{\kappa}\overline{\beta}^2$ |
| | $\Big\{\frac{3d_t-1}{2}\langle\langle c_{12}^3W_{12}^2\rangle\rangle+\overline{\alpha}(\overline{\alpha}-1)\left(5\langle\langle c_{12}^3W_{12}^2\rangle\rangle-3\langle\langle c_{12}(\mathbf{c}_{12}\cdot\mathbf{W}_{12})^2\rangle\rangle\right)+(d_t+3)\overline{\beta}(\overline{\beta}-1)\left(\langle\langle c_{12}^3W_{12}^2\rangle\rangle-\langle\langle c_{12}(\mathbf{c}_{12}\cdot\mathbf{W}_{12})^2\rangle\rangle\right)+(d_t+3)\Big[\langle\langle c_{12}^{-1}[\mathbf{C}_{12}\cdot(\mathbf{c}_{12}\times\mathbf{W}_{12})]^2\rangle\rangle$ |
| | $+\langle\langle c_{12}C_{12}^2W_{12}^2\rangle\rangle-\langle\langle c_{12}(\mathbf{C}_{12}\cdot\mathbf{W}_{12})^2\rangle\rangle\Big]+3\left(\langle\langle c_{12}^3W_{12}^2\rangle\rangle+4\langle\langle c_{12}C_{12}^2W_{12}^2\rangle\rangle\right)-\Big(\langle\langle c_{12}(\mathbf{c}_{12}\cdot\mathbf{W}_{12})^2\rangle\rangle+4\langle\langle c_{12}^{-1}C_{12}^2(\mathbf{c}_{12}\cdot\mathbf{W}_{12})^2\rangle\rangle\Big)+\frac{\theta}{\kappa}\overline{\beta}^2\Big[15\langle\langle c_{12}W_{12}^4\rangle\rangle$ |
| | $-2d_t\langle\langle c_{12}^{-1}W_{12}^2(\mathbf{c}_{12}\cdot\mathbf{W}_{12})^2\rangle\rangle-\langle\langle c_{12}^{-3}(\mathbf{c}_{12}\cdot\mathbf{W}_{12})^4\rangle\rangle\Big]\Big\}-\frac{16}{3}\frac{B_4}{B_5}\sqrt{\frac{\theta}{\kappa}}\overline{\beta}\Big[(d_t-2)\overline{\beta}+4\overline{\alpha}+(d_t+2)\Big]\langle\langle(\mathbf{C}_{12}\cdot\mathbf{c}_{12})[\mathbf{C}_{12}\cdot(\mathbf{c}_{12}\times\mathbf{W}_{12})]\rangle\rangle$ |
| $(0,4)$ | $\frac{d_t^2-1}{8}\frac{\overline{\beta}^4}{\kappa^2\theta^2}\langle\langle c_{12}^5\rangle\rangle+\frac{2}{\kappa\theta}\overline{\beta}^2\Big\{\Big[\frac{(d_t+3)(d_t+1)}{4}-\frac{\overline{\beta}}{\kappa}\frac{3d_t-1}{2}+\frac{\overline{\beta}^2}{\kappa^2}\Big(\frac{3d_t-1}{2}+d_t+3\Big)\Big]\langle\langle c_{12}^3W_{12}^2\rangle\rangle-(d_t+3)\Big(\frac{1}{4}+2\frac{\overline{\beta}}{\kappa}+\frac{\overline{\beta}^2}{\kappa^2}\Big)\langle\langle c_{12}(\mathbf{c}_{12}\cdot\mathbf{W}_{12})^2\rangle\rangle+\frac{(d_t+3)}{32}$ |
| | $\times\left(\langle\langle c_{12}^3w_{12}^2\rangle\rangle-\langle\langle c_{12}(\mathbf{c}_{12}\cdot\mathbf{w}_{12})^2\rangle\rangle\right)\Big\}+2\frac{\overline{\beta}}{\kappa}\Big\{\Big(\frac{\overline{\beta}}{\kappa}-\frac{1}{2}\Big)\Big[\frac{3(d_t+3)}{4}\left(4\langle\langle c_{12}W_{12}^4\rangle\rangle+\langle\langle c_{12}w_{12}^2W_{12}^2\rangle\rangle\right)-\frac{d_t+3}{4}\Big(4\langle\langle c_{12}^{-1}W_{12}^2(\mathbf{c}_{12}\cdot\mathbf{W}_{12})^2\rangle\rangle+\langle\langle c_{12}^{-1}w_{12}^2(\mathbf{c}_{12}\cdot\mathbf{W}_{12})^2\rangle\rangle\Big)\Big]$ |
| | $+\frac{\overline{\beta}}{\kappa}\Big[\frac{11-d_t(d_t-4)}{2}\langle\langle c_{12}(\mathbf{w}_{12}\cdot\mathbf{W}_{12})^2\rangle\rangle-(7-d_t)\langle\langle c_{12}(\mathbf{w}_{12}\cdot\mathbf{W}_{12})(\mathbf{c}_{12}\cdot\mathbf{W}_{12})(\mathbf{c}_{12}\cdot\mathbf{w}_{12})\rangle\rangle-\frac{1}{2}\langle\langle c_{12}^{-2}W_{12}^2(\mathbf{c}_{12}\cdot\mathbf{W}_{12})^2\rangle\rangle+\frac{d_t-2}{2}\Big(\langle\langle c_{12}^{-1}w_{12}^2(\mathbf{c}_{12}\cdot\mathbf{W}_{12})^2\rangle\rangle$ |
| | $+\langle\langle c_{12}^{-1}W_{12}^2(\mathbf{c}_{12}\cdot\mathbf{w}_{12})^2\rangle\rangle+\langle\langle c_{12}w_{12}^2W_{12}^2\rangle\rangle\Big)\Big]+\Big(\frac{\overline{\beta}}{\kappa}-4\frac{\overline{\beta}^2}{\kappa^2}+\frac{\overline{\beta}^3}{\kappa^3}\Big)\Big(15\langle\langle c_{12}W_{12}^4\rangle\rangle-2d_t\langle\langle c_{12}^{-1}W_{12}^2(\mathbf{c}_{12}\cdot\mathbf{W}_{12})^2\rangle\rangle-\langle\langle c_{12}^{-3}(\mathbf{c}_{12}\cdot\mathbf{W}_{12})^4\rangle\rangle\Big)\Big\}$ |
| $(2,2)$ | $\frac{d_t+3}{16}\Big[\overline{\alpha}(\overline{\alpha}-1)+\frac{d_t-1}{2}\overline{\beta}(\overline{\beta}-1)\Big]\left(4\langle\langle c_{12}^3W_{12}^2\rangle\rangle+\langle\langle c_{12}^3w_{12}^2\rangle\rangle\right)-\frac{d_t+3}{4}[\overline{\alpha}+(d_t-1)\overline{\beta}]\langle\langle c_{12}(\mathbf{c}_{12}\cdot\mathbf{C}_{12})(\mathbf{w}_{12}\cdot\mathbf{W}_{12})\rangle\rangle+\frac{\overline{\beta}^2}{\kappa\theta}\frac{d_t-1}{4}\Big\{\Big[\frac{d_t+3}{8}+\overline{\alpha}(\overline{\alpha}-1)+\frac{d_t+1}{2}\overline{\beta}(\overline{\beta}-1)\Big]\langle\langle c_{12}^5\rangle\rangle$ |
| | $+\frac{d_t+3}{2}\langle\langle c_{12}^3C_{12}^2\rangle\rangle\Big\}+\frac{\overline{\beta}^2}{\kappa^2}\Big\{\frac{d_t+3}{2}(3\langle\langle c_{12}C_{12}^2W_{12}^2\rangle\rangle-\langle\langle c_{12}^{-1}C_{12}^2(\mathbf{c}_{12}\cdot\mathbf{W}_{12})^2\rangle\rangle)+\langle\langle c_{12}^3W_{12}^2\rangle\rangle\Big[\frac{3(d_t+3)}{8}+5\overline{\alpha}(\overline{\alpha}-1)+5\frac{d_t+1}{2}\overline{\beta}(\overline{\beta}-1)+(d_t+3)\overline{\beta}^2\Big]-\Big[\frac{d_t+3}{8}+3\overline{\alpha}(\overline{\alpha}-1)$ |
| | $+2\frac{d_t+1}{2}\overline{\beta}(\overline{\beta}+1)+(d_t+3)\overline{\beta}^2\Big]\langle\langle c_{12}(\mathbf{c}_{12}\cdot\mathbf{W}_{12})^2\rangle\rangle\Big\}+2\frac{\theta}{\kappa}\overline{\beta}\Big\{\overline{\beta}\Big[\frac{\overline{\beta}}{\kappa}\Big(\frac{\overline{\beta}}{\kappa}-1\Big)\Big]\Big(15\langle\langle c_{12}W_{12}^4\rangle\rangle-2d_t\langle\langle c_{12}^{-1}W_{12}^2(\mathbf{c}_{12}\cdot\mathbf{W}_{12})^2\rangle\rangle-\langle\langle c_{12}^{-3}(\mathbf{c}_{12}\cdot\mathbf{W}_{12})^4\rangle\rangle\Big)+\frac{d_t+3}{8}\Big[4\Big(3\langle\langle c_{12}W_{12}^4\rangle\rangle$ |
| | $-\langle\langle c_{12}^{-1}W_{12}^2(\mathbf{c}_{12}\cdot\mathbf{W}_{12})^2\rangle\rangle\Big)+3\langle\langle c_{12}w_{12}W_{12}^2\rangle\rangle-\langle\langle c_{12}^{-1}w_{12}^2(\mathbf{c}_{12}\cdot\mathbf{W}_{12})^2\rangle\rangle\Big]\Big\}-\frac{\overline{\beta}}{\kappa}\Big\{\Big[\frac{3(d_t+3)}{8}+5\overline{\alpha}(\overline{\alpha}-1)+\frac{3d_t-1}{2}\overline{\beta}(\overline{\beta}-1)+\frac{d_t+3}{2}\overline{\beta}(2\overline{\beta}-1)\Big]\langle\langle c_{12}^3W_{12}^2\rangle\rangle$ |
| | $-\Big[\frac{d_t+3}{8}+3\overline{\alpha}(\overline{\alpha}-1)+\frac{d_t+3}{2}\overline{\beta}(2\overline{\beta}-1)\Big]\langle\langle c_{12}(\mathbf{c}_{12}\cdot\mathbf{W}_{12})^2\rangle\rangle+\frac{d_t+3}{2}\Big[3\langle\langle c_{12}C_{12}^2W_{12}^2\rangle\rangle-\langle\langle c_{12}^{-1}C_{12}^2(\mathbf{c}_{12}\cdot\mathbf{W}_{12})^2\rangle\rangle\Big]+\Big[\frac{3(d_t+3)}{4}-5\overline{\alpha}-(2d_t+1)\overline{\beta}\Big]\langle\langle c_{12}(\mathbf{c}_{12}\cdot\mathbf{C}_{12})(\mathbf{w}_{12}\cdot\mathbf{W}_{12})\rangle\rangle$ |
| | $-\Big[\frac{d_t+3}{4}-\overline{\alpha}-\frac{d_t+1}{2}\overline{\beta}\Big]\langle\langle c_{12}^{-1}(\mathbf{c}_{12}\cdot\mathbf{C}_{12})(\mathbf{c}_{12}\cdot\mathbf{W}_{12})(\mathbf{c}_{12}\cdot\mathbf{w}_{12})\rangle\rangle+\Big(\overline{\alpha}+\frac{d_t+1}{2}\overline{\beta}\Big)\langle\langle c_{12}(\mathbf{c}_{12}\cdot\mathbf{W}_{12})(\mathbf{w}_{12}\cdot\mathbf{C}_{12})\rangle\rangle+\Big(\overline{\alpha}+\overline{\beta}\Big)\langle\langle c_{12}(\mathbf{c}_{12}\cdot\mathbf{w}_{12})(\mathbf{C}_{12}\cdot\mathbf{W}_{12})\rangle\rangle\Big\}-\frac{d_t+3}{4}\Big[\overline{\alpha}+\frac{d_t-1}{2}\overline{\beta}\Big]$ |
| | $\times\langle\langle c_{12}(\mathbf{c}_{12}\cdot\mathbf{C}_{12})(\mathbf{w}_{12}\cdot\mathbf{W}_{12})\rangle\rangle-\frac{B_4}{3B_5}\overline{\beta}\sqrt{\frac{\theta}{\kappa}}\Big\{4(d_t+2)\langle\langle(\mathbf{w}_{12}\cdot\mathbf{W}_{12})\mathbf{C}_{12}\cdot(\mathbf{c}_{12}\times\mathbf{W}_{12})\rangle\rangle-\frac{1}{\theta}\Big[(\overline{\alpha}+\overline{\beta})\langle\langle c_{12}^2\mathbf{C}_{12}\cdot(\mathbf{c}_{12}\times\mathbf{w}_{12})\rangle\rangle+8\frac{\overline{\beta}}{\kappa}\Big(4\langle\langle(\mathbf{w}_{12}\cdot\mathbf{W}_{12})\mathbf{c}_{12}\cdot(\mathbf{C}_{12}\times\mathbf{W}_{12})\rangle\rangle$ |
| | $-\langle\langle(\mathbf{c}_{12}\cdot\mathbf{W}_{12})\mathbf{w}_{12}\cdot(\mathbf{C}_{12}\times\mathbf{W}_{12})\rangle\rangle+6\langle\langle c_{12}^{-2}(\mathbf{c}_{12}\cdot\mathbf{W}_{12})(\mathbf{c}_{12}\cdot\mathbf{w}_{12})\mathbf{c}_{12}\cdot(\mathbf{C}_{12}\times\mathbf{W}_{12})\rangle\rangle\Big)\Big]\Big\}$ |

$$\begin{aligned}\frac{\langle\langle(\mathbf{C}_{12}\cdot\mathbf{\Delta}_{12})^2\rangle\rangle}{2B_5} =&\frac{1}{8}(\overline{\alpha}-\overline{\beta})^2\langle\langle c_{12}^3C_{12}^2\rangle\rangle+\frac{1}{8}\left(3\overline{\alpha}^2+\frac{d_t^2-3}{2}\overline{\beta}^2+2d_t\overline{\alpha}\overline{\beta}\right)\langle\langle c_{12}(\mathbf{c}_{12}\cdot\mathbf{C}_{12})^2\rangle\rangle+\frac{\theta}{\kappa}\overline{\beta}^2\frac{d_t+3}{4}\\ &\times\left[\langle\langle c_{12}^{-1}[\mathbf{C}_{12}\cdot(\mathbf{c}_{12}\times\mathbf{W}_{12})]^2\rangle\rangle+\langle\langle c_{12}C_{12}^2W_{12}^2\rangle\rangle-\langle\langle c_{12}(\mathbf{C}_{12}\cdot\mathbf{W}_{12})^2\rangle\rangle\right]+\frac{2B_4}{B_5}\sqrt{\frac{\theta}{\kappa}}\overline{\beta}\\ &\times\left[\left(1-\frac{B_2}{B_4}+\frac{B_2/B_4-1}{d_t-1}\right)\overline{\beta}-2\overline{\alpha}\left(1+\frac{B_2/B_4-1}{d_t-1}\right)\right]\langle\langle(\mathbf{c}_{12}\cdot\mathbf{C}_{12})\mathbf{C}_{12}\cdot(\mathbf{c}_{12}\times\mathbf{W}_{12})\rangle\rangle, \quad (1.10f)\end{aligned}$$

$$\frac{\langle\langle(c_{12}^2+4C_{12}^2)(\mathbf{c}_{12}\cdot\mathbf{\Delta}_{12})\rangle\rangle}{2B_5}=\frac{d_t+3}{8}\left(\overline{\alpha}+\overline{\beta}\frac{d_t-1}{2}\right)\left(\langle\langle c_{12}^5\rangle\rangle+4\langle\langle c_{12}^3C_{12}^2\rangle\rangle\right), \quad (1.10g)$$

$$\frac{\langle\langle(\mathbf{C}_{12}\cdot\mathbf{\Delta}_{12})(\mathbf{c}_{12}\cdot\mathbf{C}_{12})\rangle\rangle}{2B_5}=\frac{d_t+3}{8}\left(\overline{\alpha}+\overline{\beta}\frac{d_t-1}{2}\right)\langle\langle c_{12}(\mathbf{c}_{12}\cdot\mathbf{C}_{12})^2\rangle\rangle-2\sqrt{\frac{\theta}{\kappa}}\frac{B_2}{B_3}\overline{\beta}\langle\langle(\mathbf{c}_{12}\cdot\mathbf{C}_{12})\mathbf{C}_{12}\cdot(\mathbf{c}_{12}\times\mathbf{W}_{12})\rangle\rangle, \quad (1.10h)$$

$$\begin{aligned}\frac{\langle\langle(\widehat{\boldsymbol{\sigma}}\times\mathbf{\Delta}_{12})^2(4C_{12}^2+c_{12}^2)\rangle\rangle}{2B_5}=&\overline{\beta}^2\frac{d_t+3}{4}\left\{\frac{d_t-1}{4}(4\langle\langle c_{12}^3C_{12}^2\rangle\rangle+\langle\langle c_{12}^5\rangle\rangle)+\frac{\theta}{\kappa}\left[12\langle\langle c_{12}W_{12}^2C_{12}^2\rangle\rangle+3\langle\langle c_{12}^3W_{12}^2\rangle\rangle\right.\right.\\ &\left.\left.-4\langle\langle C_{12}^2c_{12}^{-1}(\mathbf{c}_{12}\cdot\mathbf{W}_{12})^2\rangle\rangle-\langle\langle c_{12}(\mathbf{c}_{12}\cdot\mathbf{W}_{12})^2\rangle\rangle)\right]\right\}, \quad (1.11a)\end{aligned}$$

$$\begin{aligned}\frac{\langle\langle(\widehat{\boldsymbol{\sigma}}\times\mathbf{\Delta}_{12})^2[\mathbf{\Delta}_{12}^2-(\mathbf{c}_{12}\cdot\mathbf{\Delta}_{12})]\rangle\rangle}{2B_5}=&\frac{\overline{\beta}^2}{2}\left\{\overline{\alpha}(\overline{\alpha}-1)\left[\frac{d_t-1}{4}\langle\langle c_{12}^5\rangle\rangle+\frac{\theta}{\kappa}\left(5\langle\langle c_{12}^3W_{12}^2\rangle\rangle-3\langle\langle c_{12}(\mathbf{c}_{12}\cdot\mathbf{W}_{12})^2\rangle\rangle\right)\right]\right.\\ &+\overline{\beta}(\overline{\beta}-1)\left(\frac{d_t^2-1}{8}\langle\langle c_{12}^5\rangle\rangle+\frac{\theta}{\kappa}\frac{3d_t-1}{2}\langle\langle c_{12}^3W_{12}^2\rangle\rangle\right)\\ &+\overline{\beta}(2\overline{\beta}-1)\frac{\theta}{\kappa}\frac{d_t+3}{2}\left[\langle\langle c_{12}^3W_{12}^2\rangle\rangle-\langle\langle c_{12}(\mathbf{c}_{12}\cdot\mathbf{W}_{12})^2\rangle\rangle\right]+\overline{\beta}^2\frac{\theta}{\kappa}\left[\frac{3d_t-1}{2}\langle\langle c_{12}^3W_{12}^2\rangle\rangle\right.\\ &\left.\left.+\frac{2\theta}{\kappa}\left(15\langle\langle c_{12}W_{12}^4\rangle\rangle-2d_t\langle\langle c_{12}^{-1}W_{12}^2(\mathbf{c}_{12}\cdot\mathbf{W}_{12})^2\rangle\rangle-\langle\langle c_{12}^{-3}(\mathbf{c}_{12}\cdot\mathbf{W}_{12})^4\rangle\rangle\right)\right]\right\}, \quad (1.11b)\end{aligned}$$

$$\frac{\langle\langle(\mathbf{C}_{12}\cdot\mathbf{c}_{12})[\mathbf{w}_{12}\cdot(\widehat{\boldsymbol{\sigma}}\times\mathbf{\Delta}_{12})]\rangle\rangle}{2B_5}=\overline{\beta}\sqrt{\frac{\theta}{\kappa}}\frac{d_t+3}{8}\left[3\langle\langle c_{12}(\mathbf{c}_{12}\cdot\mathbf{C}_{12})(\mathbf{W}_{12}\cdot\mathbf{w}_{12})\rangle\rangle-\langle\langle c_{12}^{-1}(\mathbf{c}_{12}\cdot\mathbf{C}_{12})(\mathbf{c}_{12}\cdot\mathbf{W}_{12})(\mathbf{c}_{12}\cdot\mathbf{w}_{12})\rangle\rangle\right], \quad (1.11c)$$

$$\begin{aligned}\frac{\langle\langle(\mathbf{C}_{12}\cdot\mathbf{\Delta}_{12})[\mathbf{w}_{12}\cdot(\widehat{\boldsymbol{\sigma}}\times\mathbf{\Delta}_{12})]\rangle\rangle}{2B_5}=&\frac{1}{2}\overline{\alpha}\overline{\beta}\left\{\frac{B_2-B_4}{B_5(d_t-1)}\langle\langle c_{12}^2\mathbf{C}_{12}\cdot(\mathbf{c}_{12}\times\mathbf{w}_{12})\rangle\rangle+2\sqrt{\frac{\theta}{\kappa}}\left[\frac{5}{4}\langle\langle c_{12}(\mathbf{C}_{12}\cdot\mathbf{c}_{12})(\mathbf{W}_{12}\cdot\mathbf{w}_{12})\rangle\rangle\right.\right.\\ &-\frac{1}{4}\Big(\langle\langle c_{12}^{-1}(\mathbf{C}_{12}\cdot\mathbf{c}_{12})(\mathbf{W}_{12}\cdot\mathbf{c}_{12})(\mathbf{w}_{12}\cdot\mathbf{c}_{12})\rangle\rangle+\langle\langle c_{12}(\mathbf{C}_{12}\cdot\mathbf{w}_{12})(\mathbf{W}_{12}\cdot\mathbf{c}_{12})\rangle\rangle\\ &\left.\left.+\langle\langle c_{12}(\mathbf{c}_{12}\cdot\mathbf{w}_{12})(\mathbf{W}_{12}\cdot\mathbf{C}_{12})\rangle\rangle\Big)\right]\right\}+\frac{1}{2}\overline{\beta}^2\left\{\frac{B_4-B_2}{B_5(d_t-1)}\langle\langle c_{12}^2[\mathbf{C}_{12}\cdot(\mathbf{c}_{12}\times\mathbf{w}_{12})]\rangle\rangle\right.\\ &+\sqrt{\frac{\theta}{\kappa}}\left[\frac{2d_t+1}{2}\langle\langle c_{12}(\mathbf{C}_{12}\cdot\mathbf{c}_{12})(\mathbf{W}_{12}\cdot\mathbf{w}_{12})\rangle\rangle+\frac{1}{2}\langle\langle c_{12}(\mathbf{C}_{12}\cdot\mathbf{W}_{12})(\mathbf{c}_{12}\cdot\mathbf{w}_{12})\rangle\rangle\right.\\ &\left.-\frac{d_t+1}{4}\left(\langle\langle c_{12}^{-1}(\mathbf{c}_{12}\cdot\mathbf{C}_{12})(\mathbf{c}_{12}\cdot\mathbf{W}_{12})(\mathbf{c}_{12}\cdot\mathbf{w}_{12})\rangle\rangle+\langle\langle c_{12}(\mathbf{C}_{12}\cdot\mathbf{w}_{12})(\mathbf{W}_{12}\cdot\mathbf{c}_{12})\rangle\rangle\right)\right]\\ &-\frac{4}{3}\frac{B_4}{B_5}\frac{\theta}{\kappa}\left[4\langle\langle(\mathbf{W}_{12}\cdot\mathbf{w}_{12})[\mathbf{c}_{12}\cdot(\mathbf{C}_{12}\times\mathbf{W}_{12})]\rangle\rangle-\Big(\langle\langle(\mathbf{c}_{12}\cdot\mathbf{W}_{12})[\mathbf{w}_{12}\cdot(\mathbf{C}_{12}\times\mathbf{W}_{12})]\rangle\rangle\right.\\ &\left.\left.+2\langle\langle c_{12}^{-2}(\mathbf{c}_{12}\cdot\mathbf{W}_{12})(\mathbf{c}_{12}\cdot\mathbf{w}_{12})[\mathbf{c}_{12}\cdot(\mathbf{C}_{12}\times\mathbf{W}_{12})]\rangle\rangle\Big)\right]\right\}, \quad (1.11d)\end{aligned}$$

$$\frac{\langle\langle(4C_{12}^2+\mathbf{c}_{12}^2)\mathbf{W}_{12}\cdot(\widehat{\boldsymbol{\sigma}}\times\boldsymbol{\Delta}_{12})\rangle\rangle}{2B_5} = \overline{\beta}\sqrt{\frac{\theta}{\kappa}}\frac{d_t+3}{8}\left[3\left(4\langle\langle c_{12}C_{12}^2W_{12}^2\rangle\rangle+\langle\langle c_{12}^3W_{12}^2\rangle\rangle\right)-4\langle\langle c_{12}^{-1}C_{12}^2(\mathbf{c}_{12}\cdot\mathbf{W}_{12})^2\rangle\rangle\right.$$
$$\left.+\langle\langle c_{12}(\mathbf{c}_{12}\cdot\mathbf{W}_{12})^2\rangle\rangle\right] \tag{1.11e}$$

$$\frac{\langle\langle(\boldsymbol{\Delta}_{12}^2-\mathbf{c}_{12}\cdot\boldsymbol{\Delta}_{12})\mathbf{W}_{12}\cdot(\widehat{\boldsymbol{\sigma}}\times\boldsymbol{\Delta}_{12})\rangle\rangle}{2B_5} = \frac{\overline{\beta}}{4}\sqrt{\frac{\theta}{\kappa}}\left\{\overline{\alpha}(\overline{\alpha}-1)\left[5\langle\langle c_{12}^3W_{12}^2\rangle\rangle-3\langle\langle c_{12}(\mathbf{c}_{12}\cdot\mathbf{W}_{12})^2\rangle\rangle\right]+\overline{\beta}(\overline{\beta}-1)\frac{3d_t-1}{2}\langle\langle c_{12}^3W_{12}^2\rangle\rangle\right.$$
$$\left.+\overline{\beta}(2\overline{\beta}-1)\frac{d_t+3}{2}\left[\langle\langle c_{12}^3W_{12}^2\rangle\rangle-\langle\langle c_{12}(\mathbf{c}_{12}\cdot\mathbf{W}_{12})^2\rangle\rangle\right]\right\}$$
$$+\frac{1}{2}\overline{\beta}^3\left(\frac{\theta}{\kappa}\right)^{3/2}\left[15\langle\langle c_{12}W_{12}^4\rangle\rangle-2d_t\langle\langle c_{12}^{-1}W_{12}^2(\mathbf{c}_{12}\cdot\mathbf{W}_{12})^2\rangle\rangle-\langle\langle c_{12}^{-3}(\mathbf{c}_{12}\cdot\mathbf{W}_{12})^4\rangle\rangle\right], \tag{1.11f}$$

$$\frac{\langle\langle(4W_{12}^2+w_{12}^2)(\boldsymbol{\Delta}_{12}^2-\mathbf{c}_{12}\cdot\boldsymbol{\Delta}_{12})\rangle\rangle}{2B_5} = \frac{d_t+3}{8}\left\{\left[\overline{\alpha}(\overline{\alpha}-1)+\overline{\beta}(\overline{\beta}-1)\frac{d_t-1}{2}\right]\left(\langle\langle c_{12}^3w_{12}^2\rangle\rangle+4\langle\langle c_{12}^3W_{12}^2\rangle\rangle\right)+\right.$$
$$+2\frac{\theta}{\kappa}\overline{\beta}^2\left(3\langle\langle c_{12}W_{12}^2w_{12}^2\rangle\rangle+12\langle\langle c_{12}W_{12}^4\rangle\rangle-4\langle\langle c_{12}^{-1}W_{12}^2(\mathbf{c}_{12}\cdot\mathbf{W}_{12})^2\rangle\rangle\right.$$
$$\left.\left.-\langle\langle c_{12}^{-1}w_{12}^2(\mathbf{c}_{12}\cdot\mathbf{W}_{12})^2\rangle\rangle\right)\right\}, \tag{1.11g}$$

$$\frac{\langle\langle(\mathbf{W}_{12}\cdot\mathbf{w}_{12})(\mathbf{C}_{12}\cdot\boldsymbol{\Delta}_{12})\rangle\rangle}{2B_5} = \overline{\alpha}\frac{d_t+3}{16}\langle\langle c_{12}(\mathbf{W}_{12}\cdot\mathbf{w}_{12})(\mathbf{c}_{12}\cdot\mathbf{C}_{12})\rangle\rangle+\frac{\overline{\beta}}{2}\left[\frac{(d_t-1)(d_t+3)}{8}\langle\langle c_{12}(\mathbf{W}_{12}\cdot\mathbf{w}_{12})(\mathbf{c}_{12}\cdot\mathbf{C}_{12})\rangle\rangle\right.$$
$$\left.-2\frac{B_2}{B_5}\sqrt{\frac{\theta}{\kappa}}\langle\langle(\mathbf{W}_{12}\cdot\mathbf{w}_{12})\mathbf{C}_{12}\cdot(\mathbf{c}_{12}\times\mathbf{W}_{12})\rangle\rangle\right], \tag{1.11h}$$

$$\frac{\langle\langle(\widehat{\boldsymbol{\sigma}}\times\boldsymbol{\Delta}_{12})^4\rangle\rangle}{2B_5} = \overline{\beta}^4\frac{d_t^2-1}{16}\langle\langle c_{12}^5\rangle\rangle+\frac{\theta^2}{\kappa^2}\overline{\beta}^4\left[15\langle\langle c_{12}W_{12}^4\rangle\rangle-2d_t\langle\langle c_{12}^{-1}W_{12}^2(\mathbf{c}_{12}\cdot\mathbf{W}_{12})^2\rangle\rangle-\langle\langle c_{12}^{-3}(\mathbf{c}_{12}\cdot\mathbf{W}_{12})^4\rangle\rangle\right]$$
$$+\frac{\theta}{\kappa}\overline{\beta}^4\frac{d_t+1}{2}\left[5\langle\langle c_{12}^3W_{12}^2\rangle\rangle-3\langle\langle c_{12}(\mathbf{c}_{12}\cdot\mathbf{W}_{12})^2\rangle\rangle\right], \tag{1.12a}$$

$$\frac{\langle\langle[\mathbf{W}_{12}\cdot(\widehat{\boldsymbol{\sigma}}\times\boldsymbol{\Delta}_{12})]^2\rangle\rangle}{2B_5} = \frac{\overline{\beta}^2}{2}\left\{\frac{d_t+3}{8}\left[\langle\langle c_{12}^3W_{12}^2\rangle\rangle-\langle\langle c_{12}(\mathbf{c}_{12}\cdot\mathbf{W}_{12})^2\rangle\rangle\right]+\frac{\theta}{2\kappa}\left[15\langle\langle c_{12}W_{12}^4\rangle\rangle-2d_t\langle\langle c_{12}^{-1}W_{12}^2(\mathbf{c}_{12}\cdot\mathbf{W}_{12})^2\rangle\rangle\right.\right.$$
$$\left.\left.-\langle\langle c_{12}^{-3}(\mathbf{c}_{12}\cdot\mathbf{W}_{12})^4\rangle\rangle\right]\right\}, \tag{1.12b}$$

$$\frac{\langle\langle[\mathbf{w}_{12}\cdot(\widehat{\boldsymbol{\sigma}}\times\boldsymbol{\Delta}_{12})]^2\rangle\rangle}{2B_5} = \frac{\overline{\beta}^2}{2}\left\{\frac{(d_t+3)}{8}\left[\langle\langle c_{12}^3w_{12}^2\rangle\rangle-\langle\langle c_{12}(\mathbf{c}_{12}\cdot\mathbf{w}_{12})^2\rangle\rangle\right]+\frac{\theta}{\kappa}\left[\frac{11-d_t(d_t-4)}{2}\langle\langle c_{12}(\mathbf{w}_{12}\cdot\mathbf{W}_{12})^2\rangle\rangle\right.\right.$$
$$-(7-d_t)\langle\langle c_{12}(\mathbf{w}_{12}\cdot\mathbf{W}_{12})(\mathbf{c}_{12}\cdot\mathbf{W}_{12})(\mathbf{c}_{12}\cdot\mathbf{w}_{12})\rangle\rangle-\frac{1}{2}\langle\langle c_{12}^{-3}(\mathbf{c}_{12}\cdot\mathbf{W}_{12})^2(\mathbf{c}_{12}\cdot\mathbf{w}_{12})^2\rangle\rangle$$
$$\left.\left.+\frac{d_t-2}{2}\left(\langle\langle c_{12}^{-1}w_{12}^2(\mathbf{c}_{12}\cdot\mathbf{W}_{12})^2\rangle\rangle+\langle\langle c_{12}^{-1}W_{12}^2(\mathbf{c}_{12}\cdot\mathbf{w}_{12})^2\rangle\rangle+\langle\langle c_{12}w_{12}^2W_{12}^2\rangle\rangle\right)\right]\right\}, \tag{1.12c}$$

$$\frac{\langle\langle(4W_{12}^2+w_{12}^2)(\widehat{\boldsymbol{\sigma}}\times\boldsymbol{\Delta}_{12})^2\rangle\rangle}{2B_5} = \overline{\beta}^2\frac{d_t+3}{16}\left\{(d_t-1)\left[4\langle\langle c_{12}^3W_{12}^2\rangle\rangle+\langle\langle c_{12}^3w_{12}^2\rangle\rangle\right]+4\frac{\theta}{\kappa}\left[12\langle\langle c_{12}W_{12}^4\rangle\rangle+3\langle\langle c_{12}w_{12}^2W_{12}^2\rangle\rangle\right.\right.$$
$$\left.\left.-4\langle\langle c_{12}^{-1}W_{12}^2(\mathbf{c}_{12}\cdot\mathbf{W}_{12})^2\rangle\rangle-\langle\langle c_{12}^{-1}w_{12}^2(\mathbf{c}_{12}\cdot\mathbf{W}_{12})^2\rangle\rangle)\right]\right\}, \tag{1.12d}$$

$$\frac{\langle\!\langle (4W_{12}^2+w_{12}^2)[\mathbf{W}_{12}\cdot(\widehat{\boldsymbol{\sigma}}\times\boldsymbol{\Delta}_{12})]\rangle\!\rangle}{2B_5} = \overline{\beta}\sqrt{\frac{\theta}{\kappa}}\frac{d_t+3}{8}\left[12\langle\!\langle c_{12}W_{12}^4\rangle\!\rangle + 3\langle\!\langle c_{12}w_{12}^2W_{12}^2\rangle\!\rangle - 4\langle\!\langle c_{12}^{-1}W_{12}^2(\mathbf{c}_{12}\cdot\mathbf{W}_{12})^2\rangle\!\rangle - \langle\!\langle c_{12}^{-1}w_{12}^2(\mathbf{c}_{12}\cdot\mathbf{W}_{12})^2\rangle\!\rangle\right], \tag{1.12e}$$

$$\frac{\langle\!\langle (\mathbf{w}_{12}\cdot\mathbf{W}_{12})[\mathbf{w}_{12}\cdot(\widehat{\boldsymbol{\sigma}}\times\boldsymbol{\Delta}_{12})]\rangle\!\rangle}{2B_5} = \overline{\beta}\sqrt{\frac{\theta}{\kappa}}\frac{d_t+3}{8}\left[3\langle\!\langle c_{12}(\mathbf{w}_{12}\cdot\mathbf{W}_{12})^2\rangle\!\rangle - \langle\!\langle c_{12}^{-1}(\mathbf{w}_{12}\cdot\mathbf{W}_{12})(\mathbf{c}_{12}\cdot\mathbf{W}_{12})(\mathbf{c}_{12}\cdot\mathbf{w}_{12})\rangle\!\rangle\right], \tag{1.12f}$$

$$\frac{\langle\!\langle (\widehat{\boldsymbol{\sigma}}\times\boldsymbol{\Delta}_{12})^2[\mathbf{W}_{12}\cdot(\widehat{\boldsymbol{\sigma}}\times\boldsymbol{\Delta}_{12})]\rangle\!\rangle}{2B_5} = \overline{\beta}^3\sqrt{\frac{\theta}{\kappa}}\left\{\frac{3d_t-1}{4}\langle\!\langle c_{12}^3W_{12}^2\rangle\!\rangle - \frac{d_t-3}{4}\langle\!\langle c_{12}(\mathbf{c}_{12}\cdot\mathbf{W}_{12})^2\rangle\!\rangle + \frac{d_t+3}{2}\left[\langle\!\langle c_{12}^3W_{12}^2\rangle\!\rangle - \langle\!\langle c_{12}(\mathbf{c}_{12}\cdot\mathbf{W}_{12})^2\rangle\!\rangle\right] + \frac{\theta}{\kappa}\left[15\langle\!\langle c_{12}W_{12}^4\rangle\!\rangle - 2d_t\langle\!\langle c_{12}^{-1}W_{12}^2(\mathbf{c}_{12}\cdot\mathbf{W}_{12})^2\rangle\!\rangle - \langle\!\langle c_{12}^{-3}(\mathbf{c}_{12}\cdot\mathbf{W}_{12})^4\rangle\!\rangle\right]\right\}. \tag{1.12g}$$

Equations (1.10), (1.11), and (1.12) are related to the evaluation of $\mu_{40}$, $\mu_{22}$, and $\mu_{04}$, respectively.

### D. Useful integrals and changes of variable for two-body averages in the Sonine approximation

In this subsection we summarize the most common integral expressions appearing in the two-body averages of the collisional moments appearing in Table II, in the SA.

#### 1. *Maxwellian-type integrals $I$, $J_1$, and $J_2$*

Let us start by introducing the integrals[2]

$$I(\epsilon,p,d) \equiv \int \mathrm{d}\mathbf{x}_1 \int \mathrm{d}\mathbf{x}_2\, x_{12}^p e^{-\epsilon x_1^2 - x_2^2}, \quad \epsilon > 0, \tag{1.13}$$

$d$ being the dimension of the vector space where $\mathbf{x}$ resides. It is convenient to transform our general variables $\mathbf{x}_1$ and $\mathbf{x}_2$ (in analogy to $\mathbf{c}_1$ or $\mathbf{w}_1$, and $\mathbf{c}_2$ or $\mathbf{w}_2$, respectively) into relative and center-of-mass-like variables of the form

$$\mathbf{x}_{12} = \mathbf{x}_1 - \mathbf{x}_2, \qquad \mathbf{X}_{12} = \frac{1}{2}(\epsilon\mathbf{x}_1 + \mathbf{x}_2). \tag{1.14}$$

Therefore,

$$\mathbf{x}_1 = \frac{\mathbf{x}_{12} + 2\mathbf{X}_{12}}{1+\epsilon}, \qquad \mathbf{x}_2 = \frac{2\mathbf{X}_{12} - \epsilon\mathbf{x}_{12}}{1+\epsilon}, \tag{1.15}$$

with associated Jacobian of the transformation

$$\left|\frac{\partial(\mathbf{x}_1,\mathbf{x}_2)}{\partial(\mathbf{x}_{12},\mathbf{X}_{12})}\right| = 2^d(1+\epsilon)^{-d}, \tag{1.16}$$

Note that the original center-of-mass variable is obtained by setting $\varepsilon = 1$. Using this change and $d$-spherical coordinates, Eq. (1.13) reads

$$I(\epsilon,p,d) = (1+\epsilon)^{-d}\Omega_d^2 \int_0^\infty \mathrm{d}x_{12}\, x_{12}^{d+p-1} e^{-\frac{\epsilon}{1+\epsilon}x_{12}^2} \int_0^\infty \mathrm{d}X_{12}\, X_{12}^{d-1} e^{-\frac{4}{1+\epsilon}X_{12}^2} = \pi^d \epsilon^{-d/2}\left(\frac{1+\epsilon}{\epsilon}\right)^{p/2}\frac{\Gamma\left(\frac{d+p}{2}\right)}{\Gamma\left(\frac{d}{2}\right)}, \tag{1.17}$$

where $\Omega_d = 2\pi^{d/2}/\Gamma\left(\frac{d}{2}\right)$.

Analogously, one can obtain

$$\int \mathrm{d}\mathbf{x}_1 \int \mathrm{d}\mathbf{x}_2 \, X_{12}^p e^{-\epsilon x_1^2 - x_2^2} = \frac{1}{2^p} I(\epsilon, p, d). \tag{1.18}$$

Since Eq. (1.17) applies to any $\epsilon > 0$, we can derive with respect to $\epsilon$ and then take $\epsilon = 1$ to get

$$\int \mathrm{d}\mathbf{x}_1 \int \mathrm{d}\mathbf{x}_2 \, x_{12}^p x_1^{2q} e^{-x_1^2 - x_2^2} = (-1)^q \left[\frac{\partial^q I(\epsilon, p, d)}{\partial \epsilon^q}\right]_{\epsilon=1}, \tag{1.19a}$$

$$\int \mathrm{d}\mathbf{x}_1 \int \mathrm{d}\mathbf{x}_2 \, X_{12}^p x_1^{2q} e^{-x_1^2 - x_2^2} = (-1)^q \frac{1}{2^p} \left[\frac{\partial^q I(\epsilon, p, d)}{\partial \epsilon^q}\right]_{\epsilon=1}. \tag{1.19b}$$

Similar steps lead to

$$J_1(p,q,d) \equiv \int \mathrm{d}\mathbf{x}_1 \int \mathrm{d}\mathbf{x}_2 \, x_{12}^p X_{12}^q e^{-x_1^2 - x_2^2} = \frac{2^{\frac{p-q}{2}} \pi^d \Gamma\left(\frac{d+p}{2}\right)\left(\frac{d+q}{2}\right)}{\left[\Gamma\left(\frac{d}{2}\right)\right]^2}, \tag{1.20a}$$

$$\begin{aligned} J_2(p,q,r,d) \equiv & \int \mathrm{d}\mathbf{x}_1 \int \mathrm{d}\mathbf{x}_2 \, x_{12}^p X_{12}^q (\mathbf{x}_{12} \cdot \mathbf{X}_{12})^r e^{-x_1^2 - x_2^2} \\ = & \frac{1 + (-1)^r}{2} \frac{\Gamma\left(\frac{d}{2}\right)\Gamma\left(\frac{1+r}{2}\right)}{\sqrt{\pi}\Gamma\left(\frac{d+r}{2}\right)} J_1(p+r, q+r, d). \end{aligned} \tag{1.20b}$$

Note that $J_2(p,q,0,d) = J_1(p,q,d)$ and $J_2(p,q,r,d) = 0$ if $r =$ odd.

Let us suppose that the vectors $\mathbf{x}_1, \mathbf{x}_2 \in \mathfrak{E}^{d_1}$ and $\mathbf{y}_1, \mathbf{y}_2 \in \mathfrak{E}^{d_2}$ are all embedded in the same $d$-Euclidean space, $\mathfrak{E}^d$. Then, the following identity holds,

$$\begin{aligned} &\int \mathrm{d}\mathbf{x}_1 \int \mathrm{d}\mathbf{x}_2 \int \mathrm{d}\mathbf{y}_1 \int \mathrm{d}\mathbf{y}_2 \, x_{12}^p X_{12}^q (\mathbf{x}_{12} \cdot \mathbf{X}_{12})^r y_{12}^{p'} Y_{12}^{q'} (\mathbf{y}_{12} \cdot \mathbf{Y}_{12})^{r'} (\mathbf{x}_{12} \cdot \mathbf{Y}_{12})^k e^{-x_1^2 - x_2^2 - y_1^2 - y_2^2} \\ &= \frac{1 + (-1)^k}{2} \frac{\Gamma\left(\frac{d}{2}\right)\Gamma\left(\frac{1+k}{2}\right)}{\sqrt{\pi}\Gamma\left(\frac{d+k}{2}\right)} J_2(p+k, q, r, d_1) J_2(p', q'+k, r', d_2), \end{aligned} \tag{1.21}$$

unless $\mathfrak{E}^{d_1} \perp \mathfrak{E}^{d_2}$, in which case the integral with $k > 0$ vanishes because $\mathbf{x}_{12} \cdot \mathbf{Y}_{12} = 0$.

### 2. *Sonine integral* $I_\mathrm{S}$

The Sonine approximation of the VDF implies the action of the Sonine polynomials into the integrals involved in the two-body averages. The Sonine polynomial of degree $r$ of a scalar variable $x$ in a $d$-dimensional problem is given by

$$S_r(x) = \sum_{k=0}^{r} \frac{(-1)^k \Gamma\left(\frac{d}{2} + r\right)}{\Gamma\left(\frac{d}{2} + k\right)(r-k)!k!} x^k. \tag{1.22}$$

The first three Sonine polynomials are

$$S_0(x) = 1, \quad S_1(x) = -x + \frac{d}{2}, \quad S_2(x) = \frac{1}{2}x^2 - \frac{d+2}{2}x + \frac{d(d+2)}{8}. \tag{1.23}$$

Let us define the following integral where Sonine polynomials are involved,

$$\begin{aligned} I_\mathrm{S}(p,q,r,d) \equiv & \int \mathrm{d}\mathbf{x}_1 \int \mathrm{d}\mathbf{x}_2 \, x_{12}^p x_1^{2q} e^{-x_1^2 - x_2^2} S_r(x_1^2) \\ = & (-1)^q \sum_{k=0}^{r} \frac{\Gamma\left(\frac{d}{2} + r\right)}{\Gamma\left(\frac{d}{2} + k\right)(r-k)!k!} \left[\frac{\partial^{(q+k)} I(\epsilon, p)}{\partial \epsilon^{q+k}}\right]_{\epsilon=1}, \end{aligned} \tag{1.24}$$

where in the second step we have used Eq. (1.19a).

*3. Two-body averages in the Sonine approximation*

Within the Sonine approximation described in the main text, we can obtain

$$\begin{aligned}
\langle\!\langle c_{12}^p\rangle\!\rangle_\mathrm{S} =&\pi^{-d_t-d_r}\int d\widetilde{\mathbf{\Gamma}}_1\int d\widetilde{\mathbf{\Gamma}}_2\, c_{12}^p e^{-(c_1^2+c_2^2+w_1^2+w_2^2)}\left[1+2a_{20}S_2(c_1^2)+2a_{02}S_2(w_1^2)+2a_{11}S_1(c_1^2)S_1(w_1^2)\right.\\
&\left.+2a_{00}^{(1)}P_2(\widehat{\mathbf{c}}_1\cdot\widehat{\mathbf{w}}_1)\right]\\
=&\pi^{-d_t}\left[I(1,p,d_t)+2a_{20}I_\mathrm{S}(p,0,2,d_t)\right], \qquad (1.25)
\end{aligned}$$

where $p=$ even and in the second step we have taken into account the orthogonality relations of the Sonine polynomials. Analogously,

$$\begin{aligned}
\langle\!\langle c_{12}W_{12}^2\rangle\!\rangle_\mathrm{S} =&\frac{\pi^{-d_t-d_r}}{4}\int d\widetilde{\mathbf{\Gamma}}_1\int d\widetilde{\mathbf{\Gamma}}_2\, c_{12}W_{12}^2 e^{-(c_1^2+c_2^2+w_1^2+w_2^2)}\left[1+2a_{20}S_2(c_1^2)+2a_{02}S_2(w_1^2)+2a_{11}S_1(c_1^2)S_1(w_1^2)\right]\\
=&\frac{\pi^{-d_t-d_r}}{4}\left[I(1,1,d_t)I(1,2,d_r)+2a_{20}I_\mathrm{S}(1,0,2,d_t)I(1,2,d_r)+2a_{02}I(1,1,d_t)I_\mathrm{S}(2,0,2,d_r)\right.\\
&\left.+2a_{11}I_\mathrm{S}(1,0,1,d_t)I_\mathrm{S}(2,0,1,d_r)\right], \qquad (1.26a)
\end{aligned}$$

$$\begin{aligned}
K_1(p,q,r,s,d_t,d_r)\equiv&\langle\!\langle c_{12}^pC_{12}^q(\mathbf{c}_{12}\cdot\mathbf{C}_{12})^rW_{12}^s\rangle\!\rangle_\mathrm{S}\\
=&\frac{\pi^{-d_t-d_r}}{2^s}\left\{I_\mathrm{S}(s,0,0,d_r)\left[J_2(p,q,r,d_t)+a_{20}\Big(J_2(p,q+4,r,d_t)+J_2(p,q,r+2,d_t)\right.\right.\\
&+\frac{1}{16}J_2(p+4,q,r,d_t)+\frac{1}{2}J_2(p+2,q+2,r,d_t)-\frac{d_t+2}{4}\left(4J_2(p,q+2,r,d_t)+J_2(p+2,q,r,d_t)\right)\\
&\left.+\frac{d_t(d_t+2)}{4}J_2(p,q,r,d_t)\Big)\right]+2a_{02}J_2(p,q,r,d_t)I_\mathrm{S}(s,0,2,d_r)+a_{11}I_\mathrm{S}(s,0,1,d_r)\Big[d_tJ_2(p,q,r,d_t)\\
&\left.-2J_2(p,q+2,r,d_t)-\frac{1}{2}J_2(p+2,q,r,d_t)\Big]\right\}, \qquad (1.26b)
\end{aligned}$$

$$\begin{aligned}
\langle\!\langle c_{12}^pC_{12}^q(\mathbf{c}_{12}\cdot\mathbf{C}_{12})^rW_{12}^s(\mathbf{c}_{12}\cdot\mathbf{W}_{12})^t\rangle\!\rangle_\mathrm{S}=&\frac{d_r-1}{2}\left[\frac{(1+(-1)^t)\Gamma\left(\frac{d_t}{2}\right)\Gamma\left(\frac{t+1}{2}\right)}{2\sqrt{\pi}\Gamma\left(\frac{d_t+t}{2}\right)}K_1(p+t,q,r,s+t,d_t,d_r)\right. \qquad (1.26c)\\
&\left.+2a_{00}^{(1)}F(p,q,r,s,t,d_t,d_r)\right]. \qquad (1.26d)
\end{aligned}$$

In Eq. (1.26c),

$$\begin{aligned}
F(p,q,r,s,t,d_t,d_r)\equiv&\pi^{-d_t-d_r}\int d\widetilde{\mathbf{\Gamma}}_1\int d\widetilde{\mathbf{\Gamma}}_2\, c_{12}^pC_{12}^qW_{12}^s(\mathbf{c}_{12}\cdot\mathbf{C}_{12})^r(\mathbf{c}_{12}\cdot\mathbf{W}_{12})^te^{-c_1^2-c_2^2-w_1^2-w_2^2}P_2(\widehat{\mathbf{c}}_1\cdot\widehat{\mathbf{w}}_1)\\
=&\pi^{-d_t-d_r}\frac{1+(-1)^t}{2^{s+t+5}}\frac{t}{(1+t)(3+t)}J_2(p+t+2,q,r,3)I(1,s+t+2,3), \qquad (1.27)
\end{aligned}$$

where we have taken into account that the function $F$ is meaningful only for HS.

Furthermore, we have also faced vector products in the averages, for instance,

$$\begin{aligned}
\langle\!\langle c_{12}^{-1}[\mathbf{C}_{12}\cdot(\mathbf{c}_{12}\times\mathbf{W}_{12})]^2\rangle\!\rangle=&\langle\!\langle c_{12}C_{12}^2W_{12}^2\rangle\!\rangle-\langle\!\langle C_{12}^2c_{12}^{-1}(\mathbf{c}_{12}\cdot\mathbf{W}_{12})^2\rangle\!\rangle-\langle\!\langle c_{12}(\mathbf{C}_{12}\cdot\mathbf{W}_{12})^2\rangle\!\rangle-\langle\!\langle c_{12}^{-1}W_{12}^2(\mathbf{c}_{12}\cdot\mathbf{C}_{12})^2\rangle\!\rangle\\
&+2\langle\!\langle c_{12}^{-1}(\mathbf{c}_{12}\cdot\mathbf{C}_{12})(\mathbf{C}_{12}\cdot\mathbf{W}_{12})(\mathbf{c}_{12}\cdot\mathbf{W}_{12})\rangle\!\rangle, \qquad (1.28)
\end{aligned}$$

where we have used the identity $[\mathbf{a}\cdot(\mathbf{b}\times\mathbf{c})]^2=a^2b^2c^2-a^2(\mathbf{b}\cdot\mathbf{c})^2-b^2(\mathbf{c}\cdot\mathbf{a})^2-c^2(\mathbf{a}\cdot\mathbf{b})^2+2(\mathbf{a}\cdot\mathbf{b})(\mathbf{b}\cdot\mathbf{c})(\mathbf{c}\cdot\mathbf{a})$. From parity arguments, one can prove that

$$\langle\!\langle c_{12}^{-1}(\mathbf{c}_{12}\cdot\mathbf{C}_{12})(\mathbf{C}_{12}\cdot\mathbf{W}_{12})(\mathbf{c}_{12}\cdot\mathbf{W}_{12})\rangle\!\rangle=\langle\!\langle c_{12}^{-3}(\mathbf{c}_{12}\cdot\mathbf{C}_{12})^2(\mathbf{c}_{12}\cdot\mathbf{W}_{12})^2\rangle\!\rangle, \qquad (1.29a)$$

$$\langle\!\langle c_{12}(\mathbf{C}_{12}\cdot\mathbf{W}_{12})^2\rangle\!\rangle=\langle\!\langle C_{12}^2c_{12}^{-1}(\mathbf{c}_{12}\cdot\mathbf{W}_{12})^2\rangle\!\rangle, \qquad (1.29b)$$

$$\langle\!\langle(\mathbf{c}_{12}\cdot\mathbf{C}_{12})\mathbf{C}_{12}\cdot(\mathbf{c}_{12}\times\mathbf{W}_{12})\rangle\!\rangle=\langle\!\langle(4C_{12}^2+c_{12}^2)\mathbf{C}_{12}\cdot(\mathbf{c}_{12}\times\mathbf{W}_{12})\rangle\!\rangle=0. \tag{1.29c}$$

Some of these quantities are similar to those found in the smooth case [3], but here they are more complex due to the introduction of the angular velocities.

In the computation of $\mu_{22}$ from the Sonine approximation, one needs to deal with the generalized quantity

$$\begin{aligned}K_2(p,q,r,s,t,u,d_t,d_r)\equiv&\langle\!\langle c_{12}^pC_{12}^q(\mathbf{c}_{12}\cdot\mathbf{C}_{12})^rw_{12}^sW_{12}^t(\mathbf{w}_{12}\cdot\mathbf{W}_{12})^u\rangle\!\rangle_{\mathrm{S}}\\ =&\pi^{-d_t-d_r}\Bigg\{J_2(s,t,u,d_r)\Bigg[J_2(p,q,r,d_t)+a_{20}\Bigg(J_2(p,q+4,r,d_t)+J_2(p,q,r+2,d_t)\\ &+\frac{1}{16}J_2(p+4,q,r,d_t)+\frac{1}{2}J_2(p+2,q+2,r,d_t)-\frac{d_t+2}{4}\left(4J_2(p,q+2,r,d_t)+J_2(p+2,q,r,d_t)\right)\\ &+\frac{d_t(d_t+2)}{4}J_2(p,q,r,d_t)\Bigg)\Bigg]+a_{02}J_2(p,q,r,d_t)\Bigg(J_2(s,t+4,u,d_r)+J_2(s,t,u+2,d_r)\\ &+\frac{1}{16}J_2(s+4,t,u,d_r)+\frac{1}{2}J_2(s+2,t+2,u,d_r)-\frac{d_t+2}{4}\left(4J_2(s,t+2,u,d_r)+J_2(s+2,t,u,d_r)\right)\\ &+\frac{d_t(d_t+2)}{4}J_2(s,t,u,d_r)\Bigg)+2a_{11}\Bigg[\Bigg(J_2(p,q+2,r,d_t)+\frac{1}{4}J_2(p+2,q,r,d_t)\\ &-\frac{d_t}{2}J_2(p,q,r,d_t)\Bigg)\Bigg(J_2(s,t+2,u,d_r)+\frac{1}{4}J_2(s+2,t,u,d_r)-\frac{d_r}{2}J_2(s,t,u,d_r)\Bigg)\\ &+J_2(p,q,r+1,d_t)J_2(s,t,u+1,d_r)\Bigg]\Bigg\}.\end{aligned} \tag{1.30}$$

In particular,

$$\langle\!\langle c_{12}(\mathbf{C}_{12}\cdot\mathbf{c}_{12})(\mathbf{W}_{12}\cdot\mathbf{w}_{12})\rangle\!\rangle_{\mathrm{S}}=K_2(1,0,1,0,0,1,d_t,d_r). \tag{1.31}$$

Moreover,

$$\begin{aligned}\langle\!\langle c_{12}(\mathbf{C}_{12}\cdot\mathbf{W}_{12})(\mathbf{c}_{12}\cdot\mathbf{w}_{12})\rangle\!\rangle_{\mathrm{S}}=&\langle\!\langle c_{12}(\mathbf{C}_{12}\cdot\mathbf{w}_{12})(\mathbf{c}_{12}\cdot\mathbf{W}_{12})\rangle\!\rangle_{\mathrm{S}}\\ =&\frac{d_r-1}{54}\pi^{-6}\left[2a_{11}+5a_{00}^{(1)}\right]J_2(3,2,0,3)J_2(2,2,0,3),\end{aligned} \tag{1.32a}$$

$$\langle\!\langle c_{12}^{-1}(\mathbf{c}_{12}\cdot\mathbf{C}_{12})(\mathbf{c}_{12}\cdot\mathbf{W}_{12})(\mathbf{c}_{12}\dot{\mathbf{w}}_{12})\rangle\!\rangle_{\mathrm{S}}=\frac{d_r-1}{27}\pi^{-6}\left[a_{11}+a_{00}^{(1)}\right]J_2(3,2,0,3)J_2(2,2,0,3), \tag{1.32b}$$

$$\langle\!\langle c_{12}^{-1}w_{12}^2(\mathbf{c}_{12}\cdot\mathbf{W}_{12})^2\rangle\!\rangle_{\mathrm{S}}=\frac{d_r-1}{2}\left[\frac{1}{3}K_2(1,0,0,2,2,0,3,3)+a_{00}^{(1)}\frac{\pi^{-6}}{15}J_2(3,0,0,3)J_2(2,4,0,3)\right]. \tag{1.32c}$$

From symmetry arguments, the averages involving a power of $\mathbf{c}_{12}\cdot(\mathbf{C}_{12}\times\mathbf{W}_{12})$, $\mathbf{w}_{12}\cdot(\mathbf{C}_{12}\times\mathbf{W}_{12})$, $\mathbf{C}_{12}\cdot(\mathbf{c}_{12}\times\mathbf{w}_{12})$, or $\mathbf{W}_{12}\cdot(\mathbf{c}_{12}\times\mathbf{w}_{12})$ vanish.

## II. KULLBACK–LEIBLER DIVERGENCE-LIKE FUNCTIONAL

In order to characterize the departure of the Sonine approximation for the VDF from the Maxwellian, let us introduce the Kullback–Leibler divergence (or relative entropy) [4], i.e.,

$$\mathcal{D}_{\mathrm{KL}}\left(\phi\|\phi_{\mathrm{M}}\right)=\int\mathrm{d}\widetilde{\mathbf{\Gamma}}\,\phi(\widetilde{\mathbf{\Gamma}})\ln\frac{\phi(\widetilde{\mathbf{\Gamma}})}{\phi_{\mathrm{M}}(\widetilde{\mathbf{\Gamma}})}\approx\frac{1}{2}\int\mathrm{d}\widetilde{\mathbf{\Gamma}}\,\phi_{\mathrm{M}}(\widetilde{\mathbf{\Gamma}})\left[\frac{\phi(\widetilde{\mathbf{\Gamma}})-\phi_{\mathrm{M}}(\widetilde{\mathbf{\Gamma}})}{\phi_{\mathrm{M}}(\widetilde{\mathbf{\Gamma}})}\right]^2, \tag{2.1}$$

where in the second step we have expanded $\phi$ around $\phi_{\mathrm{M}}$, neglected terms beyond second order, and take into account that $\int\mathrm{d}\widetilde{\mathbf{\Gamma}}\left[\phi(\widetilde{\mathbf{\Gamma}})-\phi_{\mathrm{M}}(\widetilde{\mathbf{\Gamma}})\right]=0$. Inserting the Sonine expansion and using the normalization relation [see Eqs. (3.15)–(3.18) of the main text], one gets

$$\mathcal{D}_{\mathrm{KL}}\left(\phi\|\phi_{\mathrm{M}}\right)\approx\frac{1}{2}\sum_{j+k+2\ell\geq2}N_{jk}^{(\ell)}\left|a_{jk}^{(\ell)}\right|^2. \tag{2.2}$$

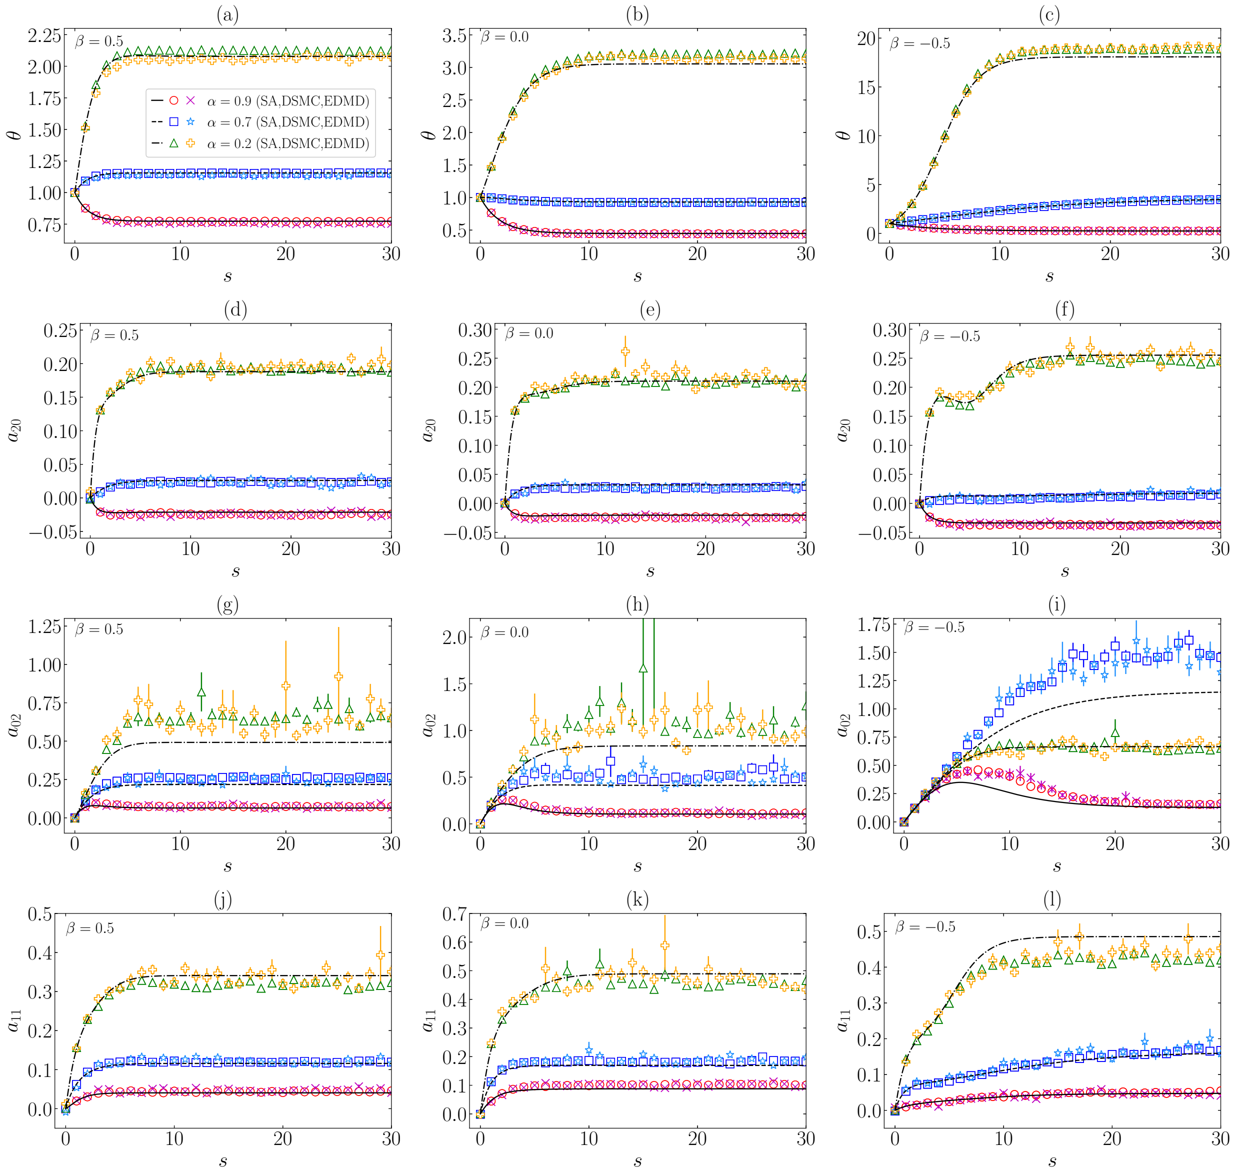

FIG. 1. Plots of (a–c) the temperature ratio $\theta(s)$, (d–f) the cumulant $a_{20}(s)$, (g–i) the cumulant $a_{02}(s)$, and (j)–(l) the cumulant $a_{11}(s)$, for uniform disks ($\kappa = \frac{1}{2}$), as functions of the number of collisions per particle $s$. The left (a, d, g, j), middle (b, e, h, k), and right (c, f, i, l) panels correspond to $\beta = 0.5$, 0, and $-0.5$, respectively. In each panel, three values of $\alpha$ are considered: 0.9 (DSMC: ○; EDMD: ×), 0.7 (DSMC: □; EDMD: ⋆), and 0.2 (DSMC: △; EDMD: +). The lines are theoretical predictions from the SA.

This gives $\mathcal{D}_{\mathrm{KL}}(\phi\|\phi_{\mathrm{M}})$ as a sum of the squares of the Sonine coefficients, weighted with the normalization constants $N_{jk}^{(\ell)}$. We now divide by the sum of the weights to define a (normalized) average as

$$\mathfrak{D}(\phi\|\phi_{\mathrm{M}}) = \frac{\sum_{j+k+2\ell\geq 2} N_{jk}^{(\ell)} \left|a_{jk}^{(\ell)}\right|^2}{\sum_{j+k+2\ell\geq 2} N_{jk}^{(\ell)}}. \tag{2.3}$$

In the Sonine approximation, $\mathfrak{D}(\phi\|\phi_{\mathrm{M}})$ becomes

$$\mathfrak{D}\left(\phi\|\phi_{\mathrm{M}}\right) = \frac{1}{N_{\mathfrak{D}}}\left[\frac{d_t(d_t+2)}{8}|a_{20}|^2 + \frac{d_r(d_r+2)}{8}|a_{02}|^2 + \frac{d_t d_r}{4}|a_{11}|^2 + (d_r-1)\frac{45}{32}\left|a_{00}^{(1)}\right|^2\right], \tag{2.4a}$$

$$N_{\mathfrak{D}} \equiv \frac{d_t + d_r}{8}(d_t + d_r + 2) + (d_r - 1)\frac{45}{32}. \tag{2.4b}$$

The Sonine approximation values of $\mathfrak{D}\left(\phi^{\mathrm{H}} \| \phi_{\mathrm{M}}\right)$ as functions of $\alpha$ and $\beta$ are plotted in Fig. 2(a) for uniform disks and in Fig. 2(b) for uniform spheres. Comparison with Figs. 2(c) and 3(c) of the main text shows that the general shape of $\mathfrak{D}\left(\phi^{\mathrm{H}} \| \phi_{\mathrm{M}}\right)$ is dominated by that of $a_{02}^{\mathrm{H}}$. We observe that the largest deviations of $\phi^{\mathrm{H}}$ from the Maxwellian distribution occur, paradoxically, in lobes emerging from a vertex at $(\alpha, \beta) = (1, -1)$. This is the region where the Sonine approximation is expected to be less reliable, at least at a quantitative level.

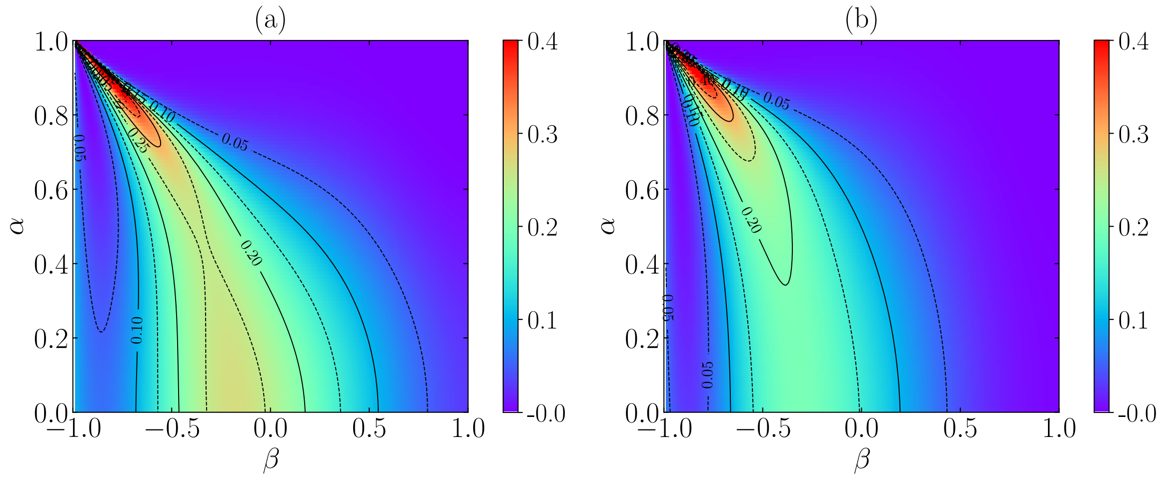


FIG. 2. Quantity $\mathfrak{D}(\phi^{\mathrm{H}} \| \phi_{\mathrm{M}})$ in the Sonine approximation as a function of $\alpha$ and $\beta$ for (a) uniform disks and (b) uniform spheres.

## III. HIGH-VELOCITY TAIL OF THE MARGINAL DISTRIBUTION $\phi_{cw}(c^2w^2)$

In this section we present an alternative justification for the high-velocity tail of $\phi_{cw}(c^2w^2)$ given in the main text.

Assuming $c \gg 1$ and $w \gg 1$ in the stationary version of the BE for the reduced VDF $\phi(\widetilde{\mathbf{\Gamma}})$, we get

$$c\frac{\partial \phi^{\mathrm{H}}}{\partial c} + w\frac{\partial \phi^{\mathrm{H}}}{\partial w} \approx -\gamma_c c \phi^{\mathrm{H}}. \tag{3.1}$$

Here, we have (i) neglected the collisional gain term versus the loss term, (ii) taken $c_{12} \to c_1$, (iii) ignored the dependence on the angle $\cos^{-1}(\widehat{\mathbf{c}} \cdot \widehat{\mathbf{w}})$ (which only exists for hard spheres), (iv) neglected $\phi^{\mathrm{H}}$ versus $c\phi^{\mathrm{H}}$, and (v) taken into account that $\mu_{20}^{\mathrm{H}}/d_t = \mu_{02}^{\mathrm{H}}/d_r$ and $\gamma_c = d_t B_1/\mu_{20}^{\mathrm{H}}$. The general solution of this linear first-order partial differential equation can be obtained from the method of characteristics as

$$\phi^{\mathrm{H}}(\widetilde{\mathbf{\Gamma}}) \approx e^{-\gamma_c c} G\left(\frac{w}{c}\right), \tag{3.2}$$

where $G(y)$ is an unknown function. Now we take the liberty of assuming that the tails of the marginal distributions $\phi_{\mathbf{w}}(\mathbf{w})$ and $\phi_{c^2w^2}(x)$ can be obtained from Eq. (3.2), i.e.,

$$\phi_{\mathbf{w}}(\mathbf{w}) \approx \Omega_{d_t} \int_0^\infty \mathrm{d}c\, c^{d_t-1} e^{-\gamma_c c} G\left(\frac{w}{c}\right), \tag{3.3a}$$

$$\phi_{cw}(x) \approx \frac{\Omega_{d_t}\Omega_{d_r}}{2} x^{\frac{d_r}{2}-1} \int_0^\infty \mathrm{d}c\, c^{d_t-d_r-1} e^{-\gamma_c c} G\left(\frac{\sqrt{x}}{c^2}\right). \tag{3.3b}$$

Consistency of Eq. (3.3a) with the high-velocity tail $\phi_{\mathbf{w}}(\mathbf{w}) \sim w^{-\gamma_w}$ implies that $G(y) \sim y^{-\gamma_w}$ for large $y$. Insertion of this asymptotic form of $G(y)$ into Eq. (3.3b) finally yields

$$\phi_{cw}^{\mathrm{H}}(x) \sim x^{-\gamma_{cw}}, \quad \gamma_{cw} = 1 + \frac{\gamma_w - d_r}{2}, \tag{3.4}$$

in agreement with the result in the main text.

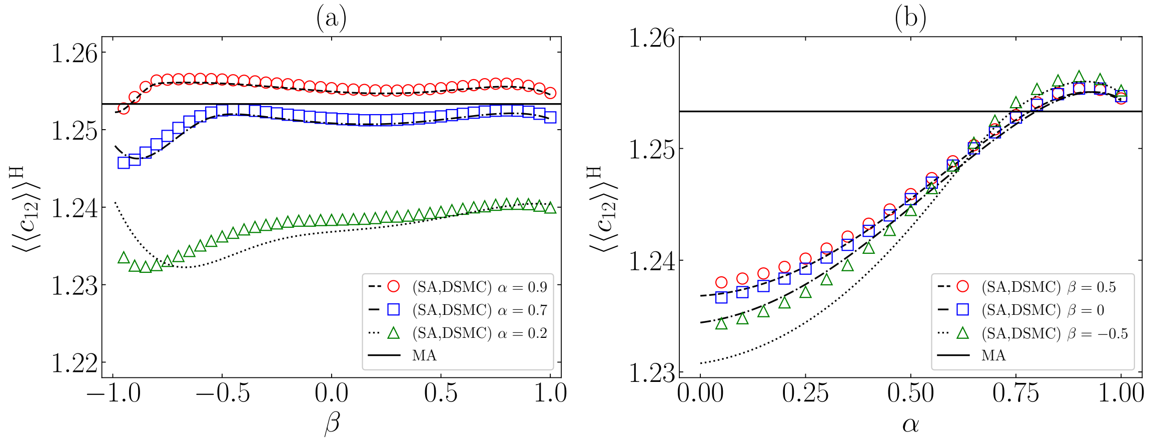


FIG. 3. Two-body average $\langle\langle c_{12}\rangle\rangle^{\rm H}$ from Maxwellian and Sonine approximations (lines) and DSMC simulation outcomes (symbols) for uniform disks ($\kappa = \frac{1}{2}$) as a function of (a) the coefficient of tangential restitution $\beta$ (at $\alpha = 0.9$, 0.7, and 0.2), (b) the coefficient of normal restitution $\alpha$ (at $\beta = 0.5$, 0, and $-0.5$).

## IV. TRANSIENT STATES

In the main text, we focused on the comparison between the theoretical predictions and the simulation data for the HCS. As a complement, here we provide a comparison for the temporal evolution toward the HCS.

Figure 1 shows the evolution of $\theta(s)$, $a_{20}(s)$, $a_{02}(s)$, and $a_{11}(s)$, starting from a Maxwellian and equipartioned initial state, so that $\theta(0) = 1$ and $a_{20}(0) = a_{02}(0) = a_{11}(0) = 0$. We observe that the Sonine-approximation theoretical predictions agree very well with simulations, except close to the HCS values for the cases in which $a_{02}^{\rm H}$, $a_{11}^{\rm H} \sim \mathcal{O}(1)$.

## V. COMPUTATION OF $\langle\langle c_{12}\rangle\rangle^{\rm H}$, $\mu_{20}^{\rm H}$, AND $\mu_{02}^{\rm H}$ FROM DSMC. COMPARISON WITH THE MAXWELLIAN AND SONINE APPROXIMATIONS

An important point of our work is the exact expression—in the framework of the BE—of the relevant collisional moments in terms of two-body averages, as displayed in Table II. It is then interesting to compute the HCS collisional moments $\mu_{20}^{\rm H}$ and $\mu_{02}^{\rm H}$ from DSMC and compare the results with predictions from the Maxwellian and Sonine approximations.

Before starting with the collisional moments, let us first consider the simple two-body average $\langle\langle c_{12}\rangle\rangle$. It can be computed in simulations as

$$\langle\langle c_{12}\rangle\rangle = \frac{1}{N'}\sum_{ij}^{N'} c_{ij}, \tag{5.1}$$

with, in principle, $N' = N(N-1)/2$ being the total number of pairs. Since we had $N = 10^4$ particles, this would imply $N' \simeq 5\times 10^7$ pairs. Instead, in order to accelerate the computation, we took a random sample of $N' = 10^5$ pairs, which represent a 2% of the total number of pairs. The results for $\langle\langle c_{12}\rangle\rangle^{\rm H}$ are displayed in Fig. 3. While the Maxwellian-approximation value, $\langle\langle c_{12}\rangle\rangle_{\rm M} = \sqrt{\pi/2} \simeq 1.253$, is independent of $\alpha$ and $\beta$, the dependence of $\langle\langle c_{12}\rangle\rangle^{\rm H}$ on both coefficients of restitution is well predicted by the Sonine approximation, at least semi-quantitatively.

Now we turn to the collisional moments $\mu_{20}$ and $\mu_{02}$, whose expressions as linear combinations of the three two-body averages $\langle\langle c_{12}^3\rangle\rangle$, $\langle\langle c_{12}W_{12}^2\rangle\rangle$, and $\langle\langle c_{12}^{-1}(\mathbf{c}_{12}\cdot\mathbf{W}_{12})^2\rangle\rangle$ are displayed in Table II. Those two-body averages are evaluated by the DSMC method by sums over pairs analogous to Eq. (5.1), again with $N' = 10^5$. From Figs. 4(a–d), we infer that both Maxwellian and, especially, Sonine approximation provide good estimates of the two first collisional moments $\mu_{20}^{\rm H}$ and $\mu_{02}^{\rm H}$. Moreover, as Figs. 4(e, f) show, the HCS condition $\mu_{20}^{\rm H}/2\mu_{02}^{\rm H} = 1$ is very accurately fulfilled by the DSMC data.

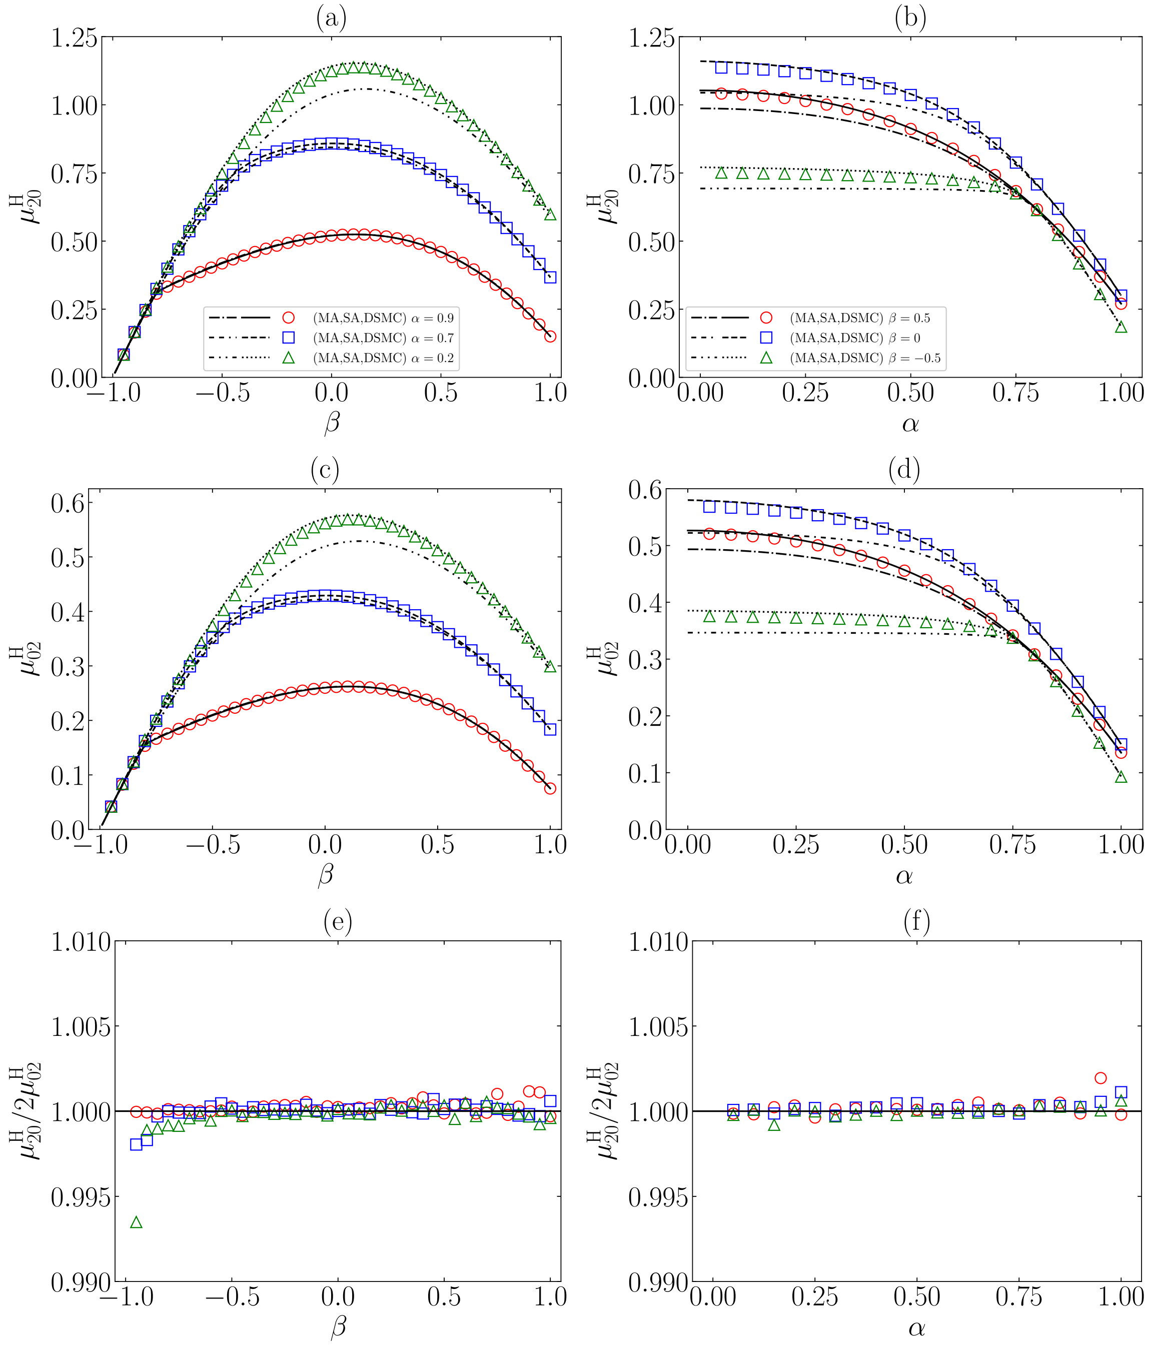


FIG. 4. Plots of (a, b) the collisional moment $\mu_{20}^{\rm H}$, (c, d) the collisional moment $\mu_{02}^{\rm H}$, and (e, f) the ratio $\mu_{20}^{\rm H}/2\mu_{02}^{\rm H}$ for uniform disks ($\kappa=\frac{1}{2}$). The quantities are plotted versus (a, c, e) the coefficient of tangential restitution $\beta$ (at $\alpha=0.9$, 0.7, and 0.2) and (b, d, f) the coefficient of normal restitution $\alpha$ (at $\beta=0.5$, 0, and $-0.5$). Symbols represent DSMC values and lines in panels (a–d) correspond to the Sonine-approximation predictions. The thick black lines in panels (e, f) represent the HCS condition $\mu_{20}^{\rm H}/2\mu_{02}^{\rm H}=1$.

## VI. SOME TECHNICAL DETAILS ABOUT THE HIGH-VELOCITY FITTING

### A. Fitting of the exponents $\gamma_c$, $\gamma_w$, and $\gamma_{cw}$

To get the high-velocity tail exponents $\gamma_c$, $\gamma_w$, and $\gamma_{cw}$ from simulations (see Fig. 9 of the main text), we fitted the data according to some conditions. First of all, we defined threshold values for the velocity variables $x=c,w,c^2w^2$,

beyond which the velocities were considered high enough as to observe the asymptotic behavior. Those thresholds are defined as $x_{\text{thres}} = \max\{\widetilde{x}, x_*^{\text{M}}\}$, where the values of $\widetilde{x}$ are

$$\widetilde{c} = \frac{5/2}{\sqrt{\dfrac{\overline{\alpha}^2}{2\alpha^2} + \dfrac{\overline{\beta}^2}{2\beta^2}}}, \quad \widetilde{w} = \frac{5}{2}\frac{\kappa|\beta|}{\overline{\beta}}, \quad \widetilde{c^2w^2} = \widetilde{c}^2\widetilde{w}^2. \tag{6.1}$$

This ensures that $c_2'' \gg 1$ and $w_2'' \gg 1$ in Eqs. (B2) and (B4) of the main text. In what concerns to the values of $x_*^{\text{M}}$, they were determined under the condition of fulfilling a continuous and differentiable match between the Maxwellian approximation VDF and the high-velocity tail behavior, as derived in Section VI B.

For each histogram, we firstly chose the range of points comprised between $x_{\text{thres}}$ and $x_{\max}$, where $x_{\max}$ represents the maximum value of $x$ in our dataset for a given system. If $x_{\max} < x_{\text{thres}}$, we concluded that there were not enough data to get a trusted fitting. On the other hand, if $x_{\max} > x_{\text{thres}}$, we proceeded to choose the proper subrange of data to be fitted from a minimization of $|\chi^2/\text{d.o.f} - 1|$,[5] where $\chi^2$ is the *chi-square* statistic (computed assuming diagonal covariance) and d.o.f is the number of degrees of freedom of the fit. If the number of points in the subrange were larger than 5, we fitted them to the desirable form, getting the slope, as well as the standard deviation of the chosen points in the dataset with respect to the fitting parameters. Finally, we computed Pearson's coefficient of determination, $R^2$, concluding that the fit was trustable if $R^2 \geq 0.9$, discarding the results otherwise.

### B. Matching points $x_*^{\text{M}}$

In previous works for the smooth case [6], a merged HCS VDF was built from a match of the thermal part (as described by the Sonine approximation) and the asymptotic tail, the matching point $c_*$ being determined by imposing continuity of the VDF and of its first derivative. In our work, we used this same method to compute the matching points $x_*$ for the marginal distributions $\phi_{\mathbf{c}}^{\text{H}}$, $\phi_{\mathbf{w}}^{\text{H}}$, and $\phi_{cw}^{\text{H}}$.

Although we present below the derivation of $x_*$ from the Sonine approximation, we actually considered in the fitting the matching points $x_*^{\text{M}}$ provided by the MA. This is due to the appearance of bimodal thermal regions of the VDF (especially for $\phi_{\mathbf{w}}^{\text{H}}$) in the Sonine approximation, not observed in simulations, and even unphysical negative values in a small range of values, as previously reported for HS.[1] We exclusively show below the results for hard disks ($d_t = 2$, $d_r = 1$).

#### 1. *Matching of $\phi_{\mathbf{c}}^{\text{H}}(\mathbf{c})$: $c_*^{\text{M}}$*

We construct a merged distribution $\phi_{\mathbf{c}}^{\text{H}}(\mathbf{c})$, such that it coincides with that of the Sonine approximation for $c < c_*$ and with its asymptotic high-velocity tail for $c > c_*$, i.e.,

$$\phi_{\mathbf{c}}^{\text{H}}(\mathbf{c}) = \mathcal{A}_c^{\text{th}} e^{-c^2}\left[1 + a_{20}^{\text{H}} S_2(c^2)\right]\Theta(c_* - c) + \mathcal{A}_c e^{-\gamma_c c}\Theta(c - c_*). \tag{6.2}$$

Imposing the continuity of $\phi_{\mathbf{c}}^{\text{H}}(\mathbf{c})$ and its first derivative at the matching point $c_*$ yields the following 5th-degree polynomial equation:

$$c_* = \frac{\gamma_c}{2} - \frac{a_{20}^{\text{H}} c_*(c_* - 2)}{1 + a_{20}^{\text{H}} S_2(c_*^2)}. \tag{6.3}$$

As said above, however, we take the Maxwellian approximation for the thermal part ($c < c_*$), i.e., $c_*^{\text{M}} = \gamma_c/2$.

#### 2. *Matching of $\phi_{\mathbf{w}}^{\text{H}}(\mathbf{w})$: $w_*^{\text{M}}$*

In this case, we have

$$\phi_{\mathbf{w}}^{\text{H}}(\mathbf{w}) = \mathcal{A}_w^{\text{th}} e^{-w^2}\left[1 + a_{02}^{\text{H}} S_2(w^2)\right]\Theta(w_* - w) + \mathcal{A}_w w^{-\gamma_w}\Theta(w - w_*). \tag{6.4}$$

Again, we assume continuity of the function and its first derivative at $w^*$, which gives a cubic equation for $w_*^2$,

$$w_*^2 = \frac{\gamma_w}{2} - \frac{a_{02}^{\text{H}} w_*^2\left(3 - 2w_*^2\right)}{1 + a_{02}^{\text{H}} S_2(w_*^2)}. \tag{6.5}$$

Thus, $w_*^{\text{M}} = \sqrt{\gamma_w/2}$.

### 3. Matching of $\phi^{\mathrm{H}}_{c^2w^2}(x)$: $x_*^{\mathrm{M}}$

The merged function is now

$$\phi^{\mathrm{H}}_{cw}(x) = \mathcal{A}^{\mathrm{th}}_{cw} x^{-\frac{1}{2}} e^{-2\sqrt{x}} \left(1 + \frac{16a^{\mathrm{H}}_{20} + 4a^{\mathrm{H}}_{11} + 6a^{\mathrm{H}}_{02}}{8} - \sqrt{x}\frac{5a^{\mathrm{H}}_{20} + 6a^{\mathrm{H}}_{11} + 5a^{\mathrm{H}}_{02}}{4} + x\frac{a^{\mathrm{H}}_{20} + 2a^{\mathrm{H}}_{11} + a^{\mathrm{H}}_{02}}{2}\right)\Theta(x_* - x) + \mathcal{A}_{cw} x^{-\gamma_{cw}}\Theta(x - x_*), \tag{6.6}$$

where we have used $K_{\frac{1}{2}}(2\sqrt{x}) = \sqrt{\pi}e^{-2\sqrt{x}}/2x^{1/4}$. From the continuity conditions one gets the cubic equation

$$x_*^{3/2}\left(a^{\mathrm{H}}_{20} + 2a^{\mathrm{H}}_{11} + a^{\mathrm{H}}_{02}\right) - x_*\left[\left(a^{\mathrm{H}}_{20} + a^{\mathrm{H}}_{02}\right)(3 + \gamma_{cw}) + a^{\mathrm{H}}_{11}(2 + \gamma_{cw})\right] + x_*^{1/2}\left[2 + a^{\mathrm{H}}_{20}\left(4 + \frac{5\gamma_{cw}}{2}\right) + a^{\mathrm{H}}_{11}(1 + 3\gamma_{cw}) + \frac{a^{\mathrm{H}}_{02}}{2}(3 + 5\gamma_{cw})\right] - (2\gamma_{cw} - 1)\left[1 + 2a^{\mathrm{H}}_{20} + \frac{1}{2}a^{\mathrm{H}}_{11} + \frac{3}{4}a^{\mathrm{H}}_{02}\right] = 0. \tag{6.7}$$

$$(2\gamma_{cw} - 1)\left(1 + 2a^{\mathrm{H}}_{20} + \frac{1}{2}a^{\mathrm{H}}_{11} + \frac{3}{4}a^{\mathrm{H}}_{02}\right) = x_*^{3/2}\left(a^{\mathrm{H}}_{20} + 2a^{\mathrm{H}}_{11} + a^{\mathrm{H}}_{02}\right) - x_*\left[\left(a^{\mathrm{H}}_{20} + a^{\mathrm{H}}_{02}\right)(3 + \gamma_{cw}) + a^{\mathrm{H}}_{11}(2 + \gamma_{cw})\right] + x_*^{1/2}\left[2 + a^{\mathrm{H}}_{20}\left(4 + \frac{5\gamma_{cw}}{2}\right) + a^{\mathrm{H}}_{11}(1 + 3\gamma_{cw}) + \frac{a^{\mathrm{H}}_{02}}{2}(3 + 5\gamma_{cw})\right]. \tag{6.8}$$

In the Maxwellian approximation, we simply get $x_*^{\mathrm{M}} = \left(\gamma_{cw} - \frac{1}{2}\right)^2$.

---


[1] F. Vega Reyes, A. Santos, and G. M. Kremer, Role of roughness on the hydrodynamic homogeneous base state of inelastic spheres, Phys. Rev. E **89**, 020202(R) (2014).

[2] V. Garzó, *Granular Gaseous Flows. A Kinetic Theory Approach to Granular Gaseous Flows* (Springer Nature, Switzerland, 2019).

[3] N. V. Brilliantov and T. Pöschel, *Kinetic Theory of Granular Gases* (Oxford University Press, Oxford, 2004).

[4] A. Megías and A. Santos, Kullback–Leibler divergence of a freely cooling granular gas, Entropy **22**, 1308 (2020).

[5] P. Young, *Everything You Wanted to Know About Data Analysis and Fitting but Were Afraid to Ask*, SpringerBriefs in Physics (Springer, Cham, 2015).

[6] T. Pöschel, N. V. Brilliantov, and A. Formella, Impact of high-energy tails on granular gas properties, Phys. Rev. E **74**, 041302 (2006).
